# Supplementary material for: Global Extraction of the $\rm^{12}C$ Nuclear Electromagnetic Response Functions (${\cal R}_L$ and ${\cal R}_T$) and Comparisons to Nuclear Theory and Neutrino/Electron Monte Carlo Generators
Source: arXiv:2409.10637 source file (2025-08-05)

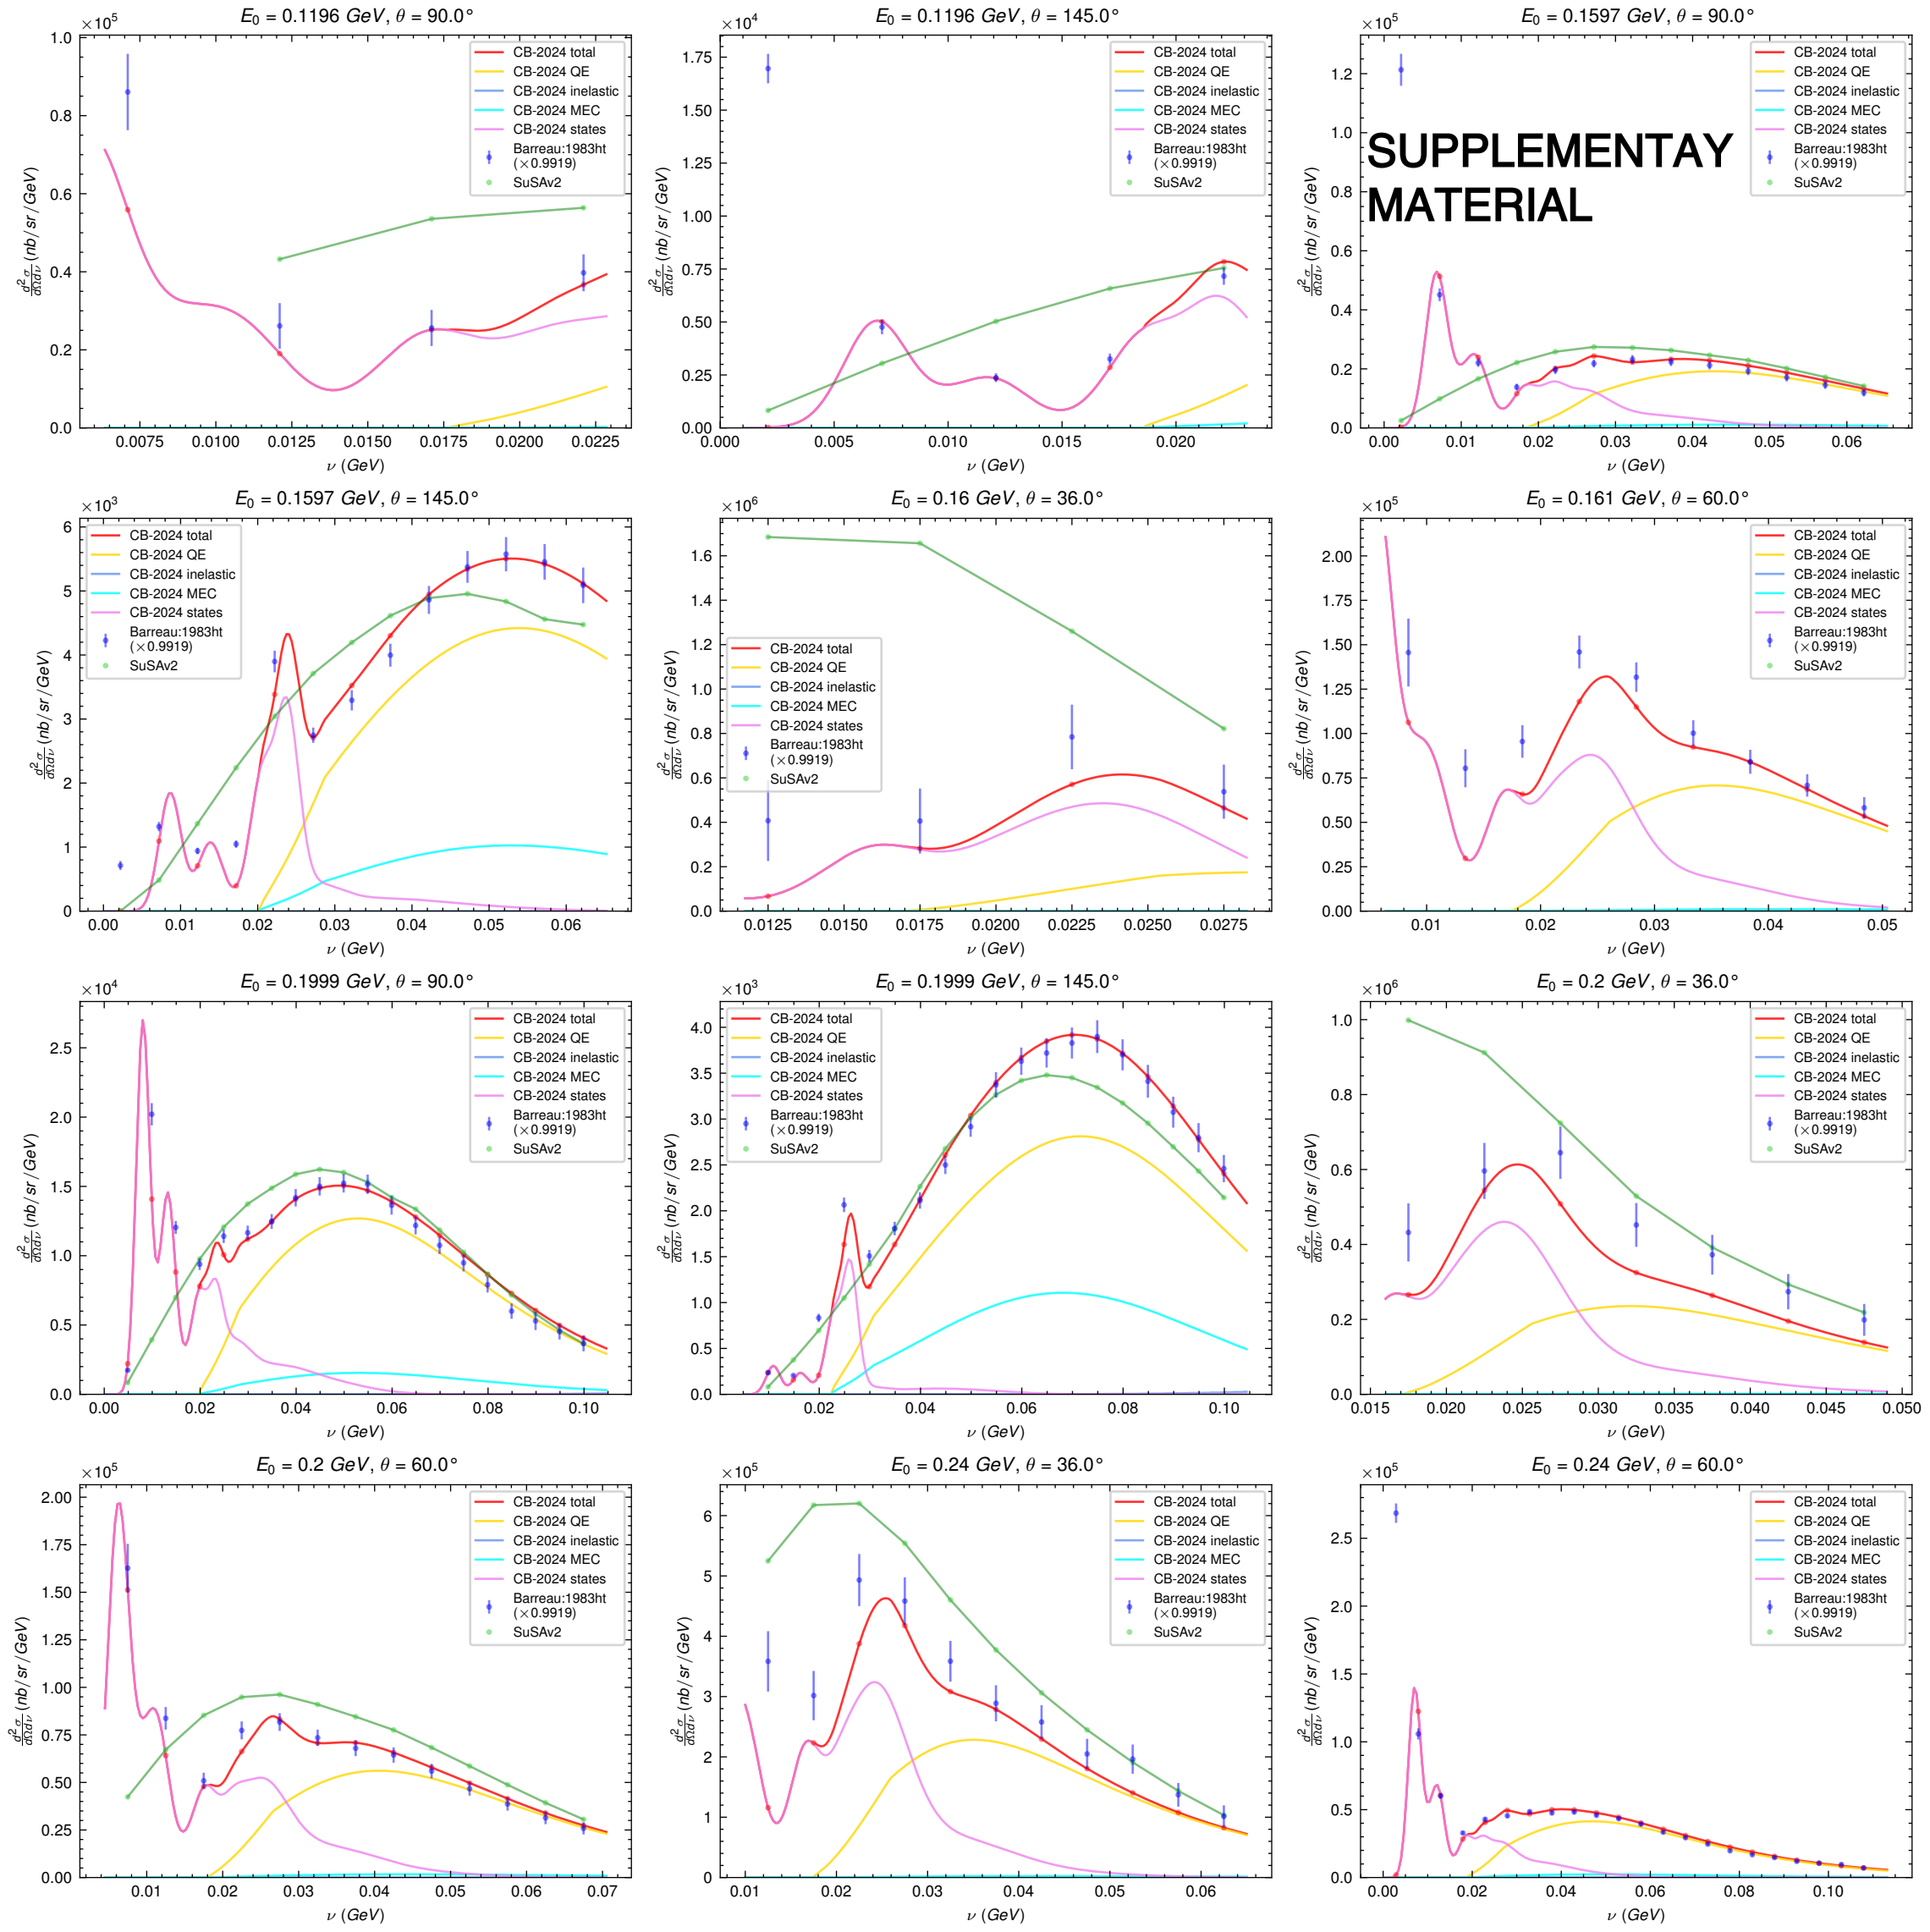

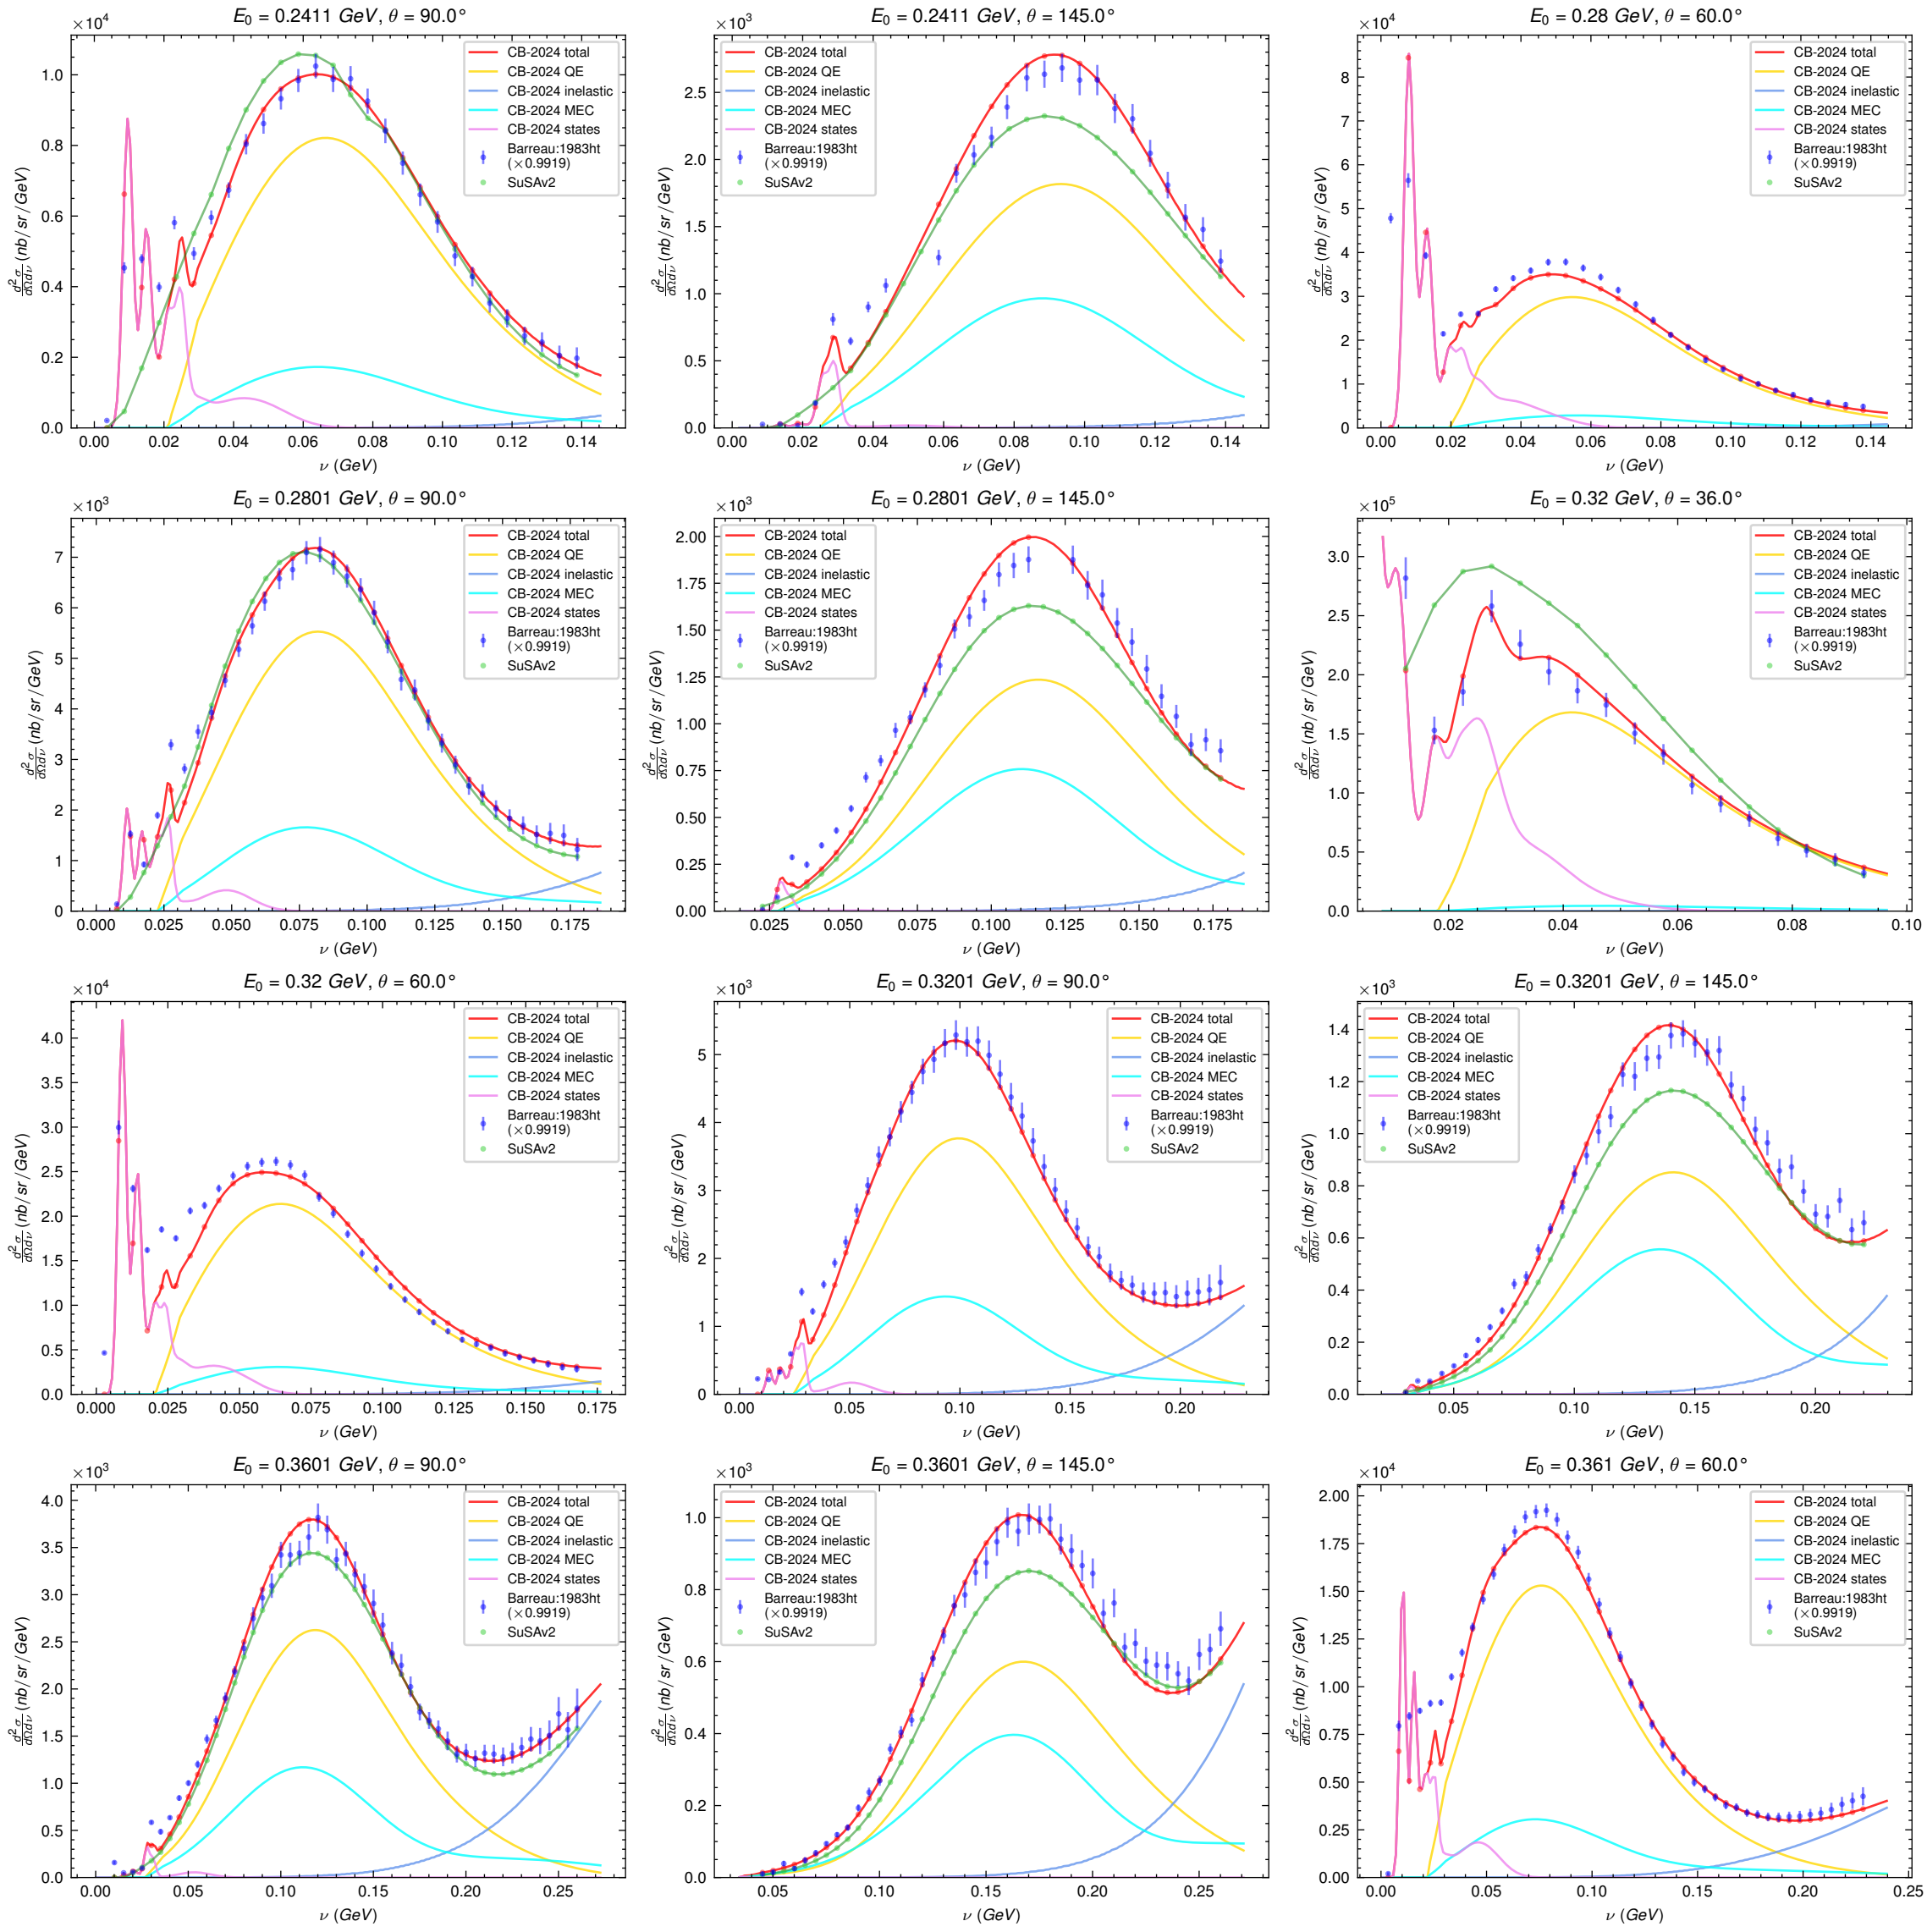

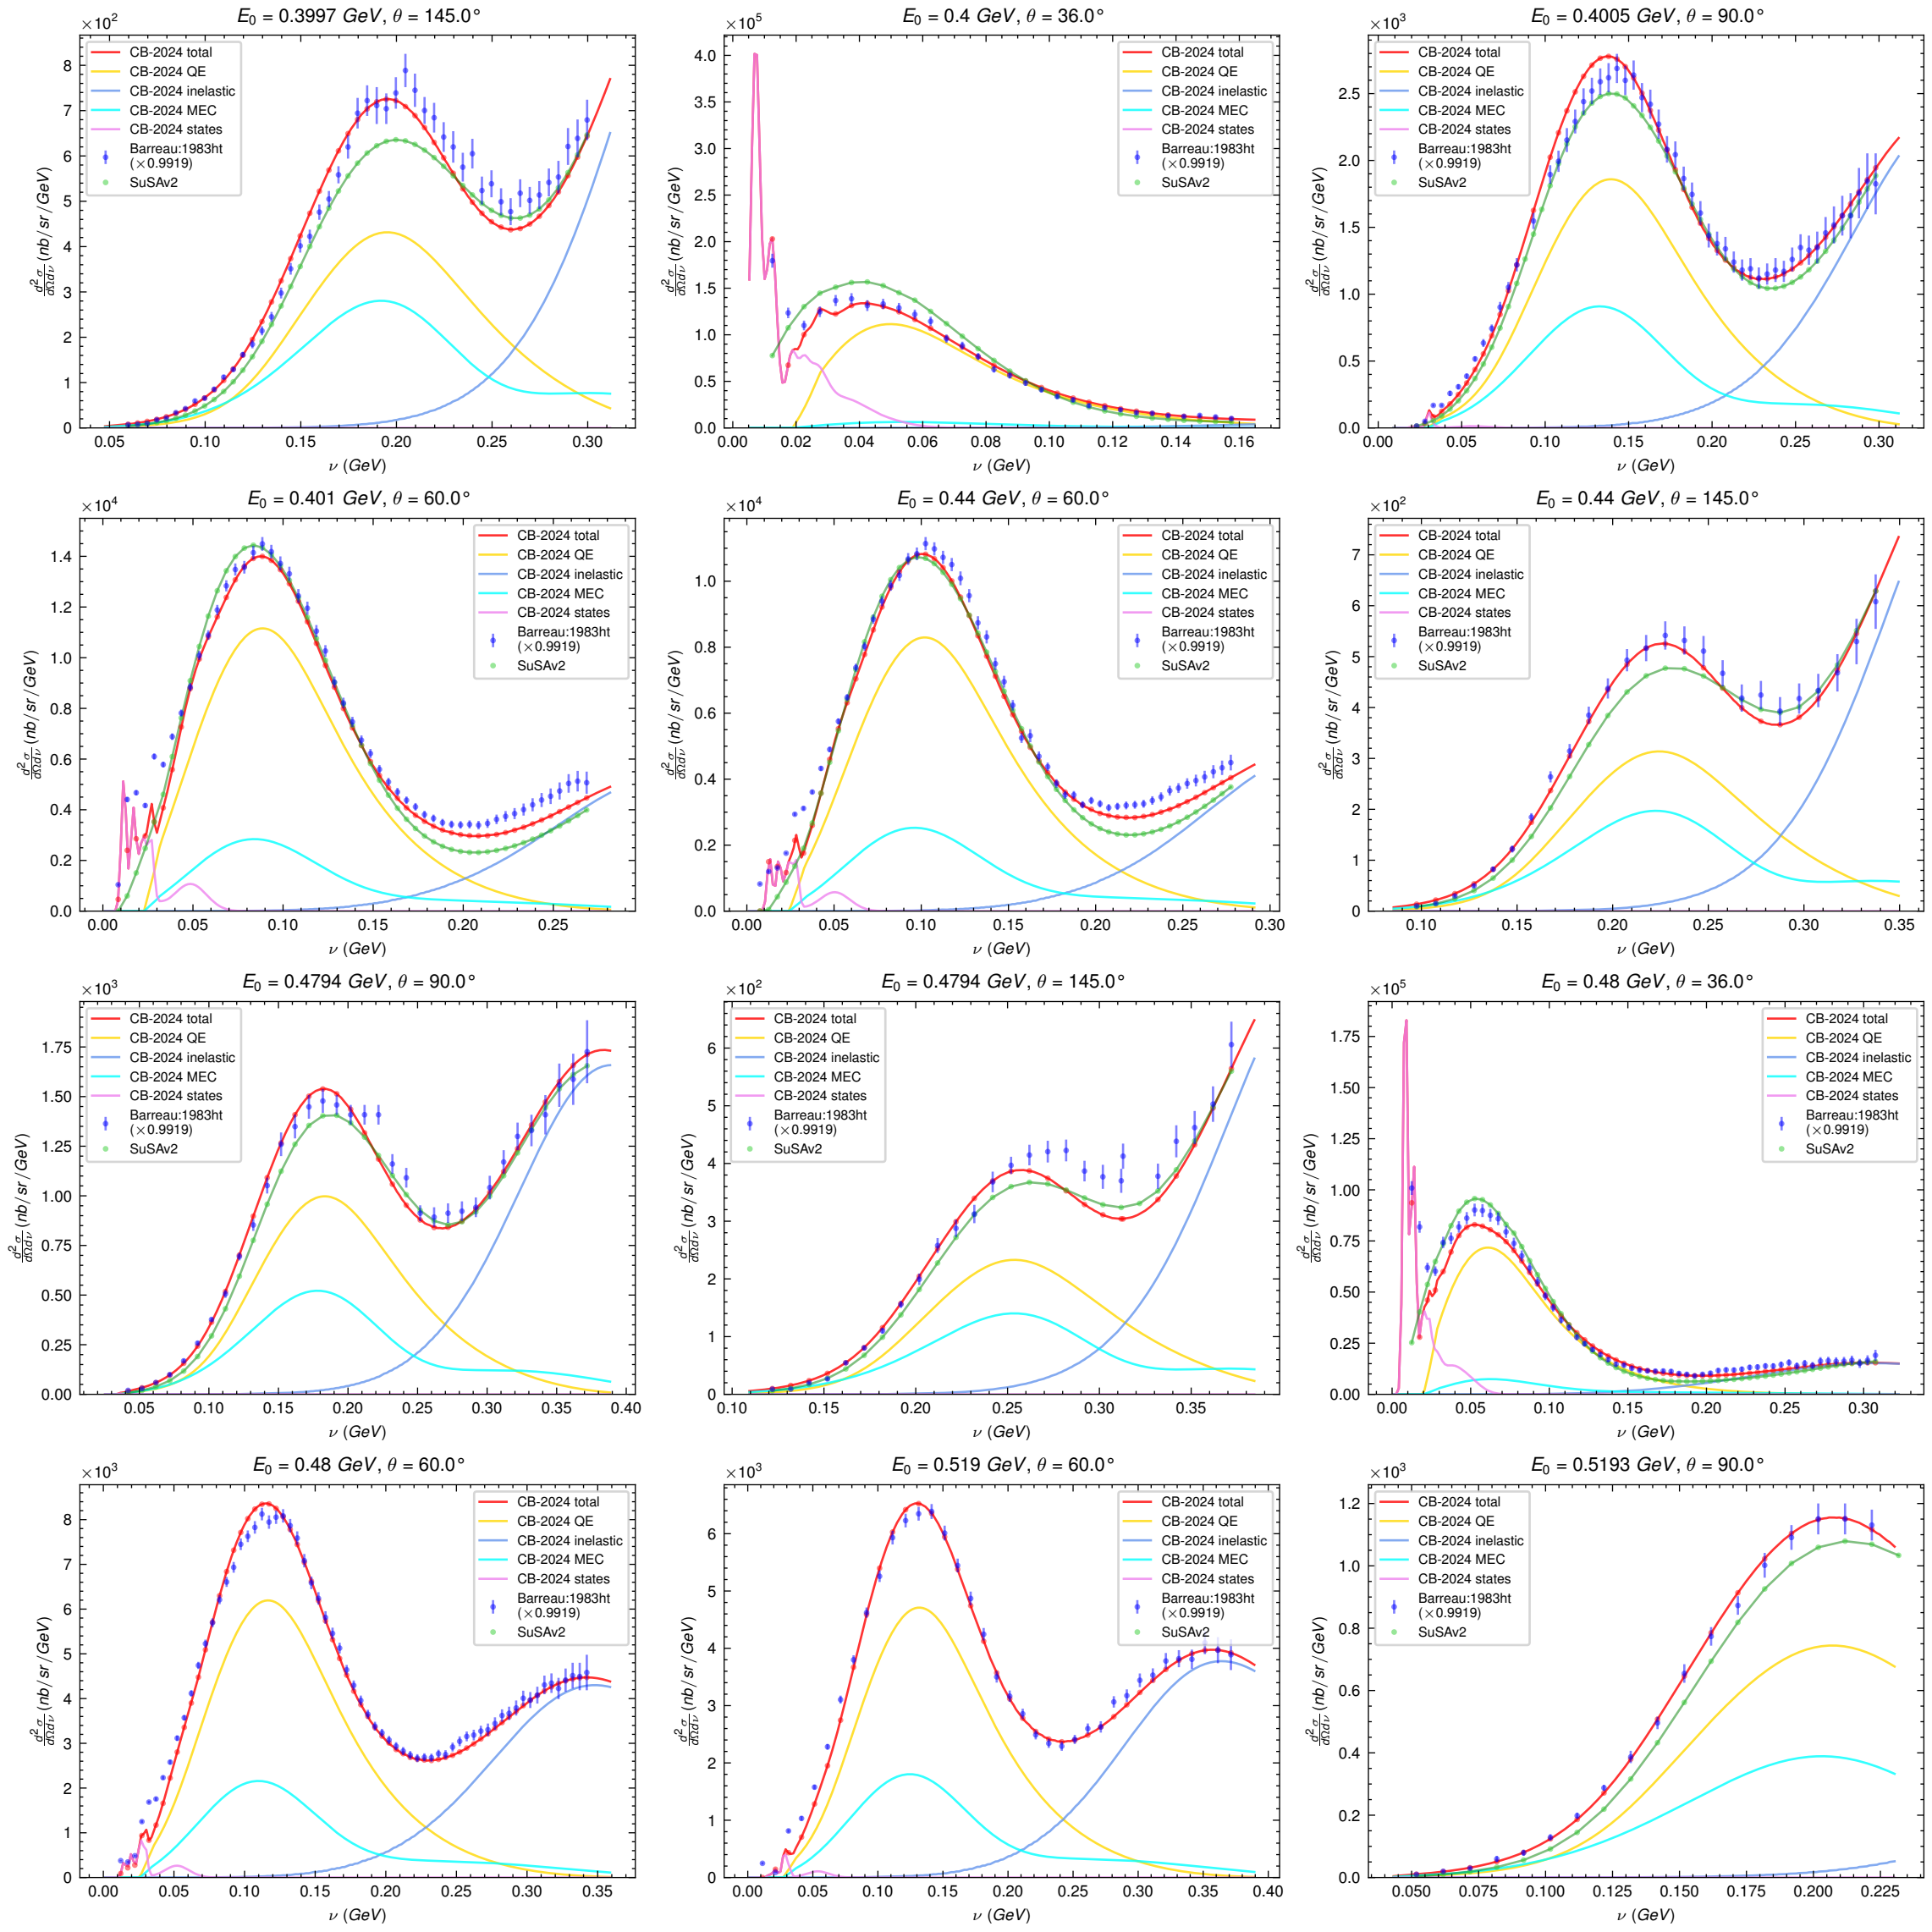

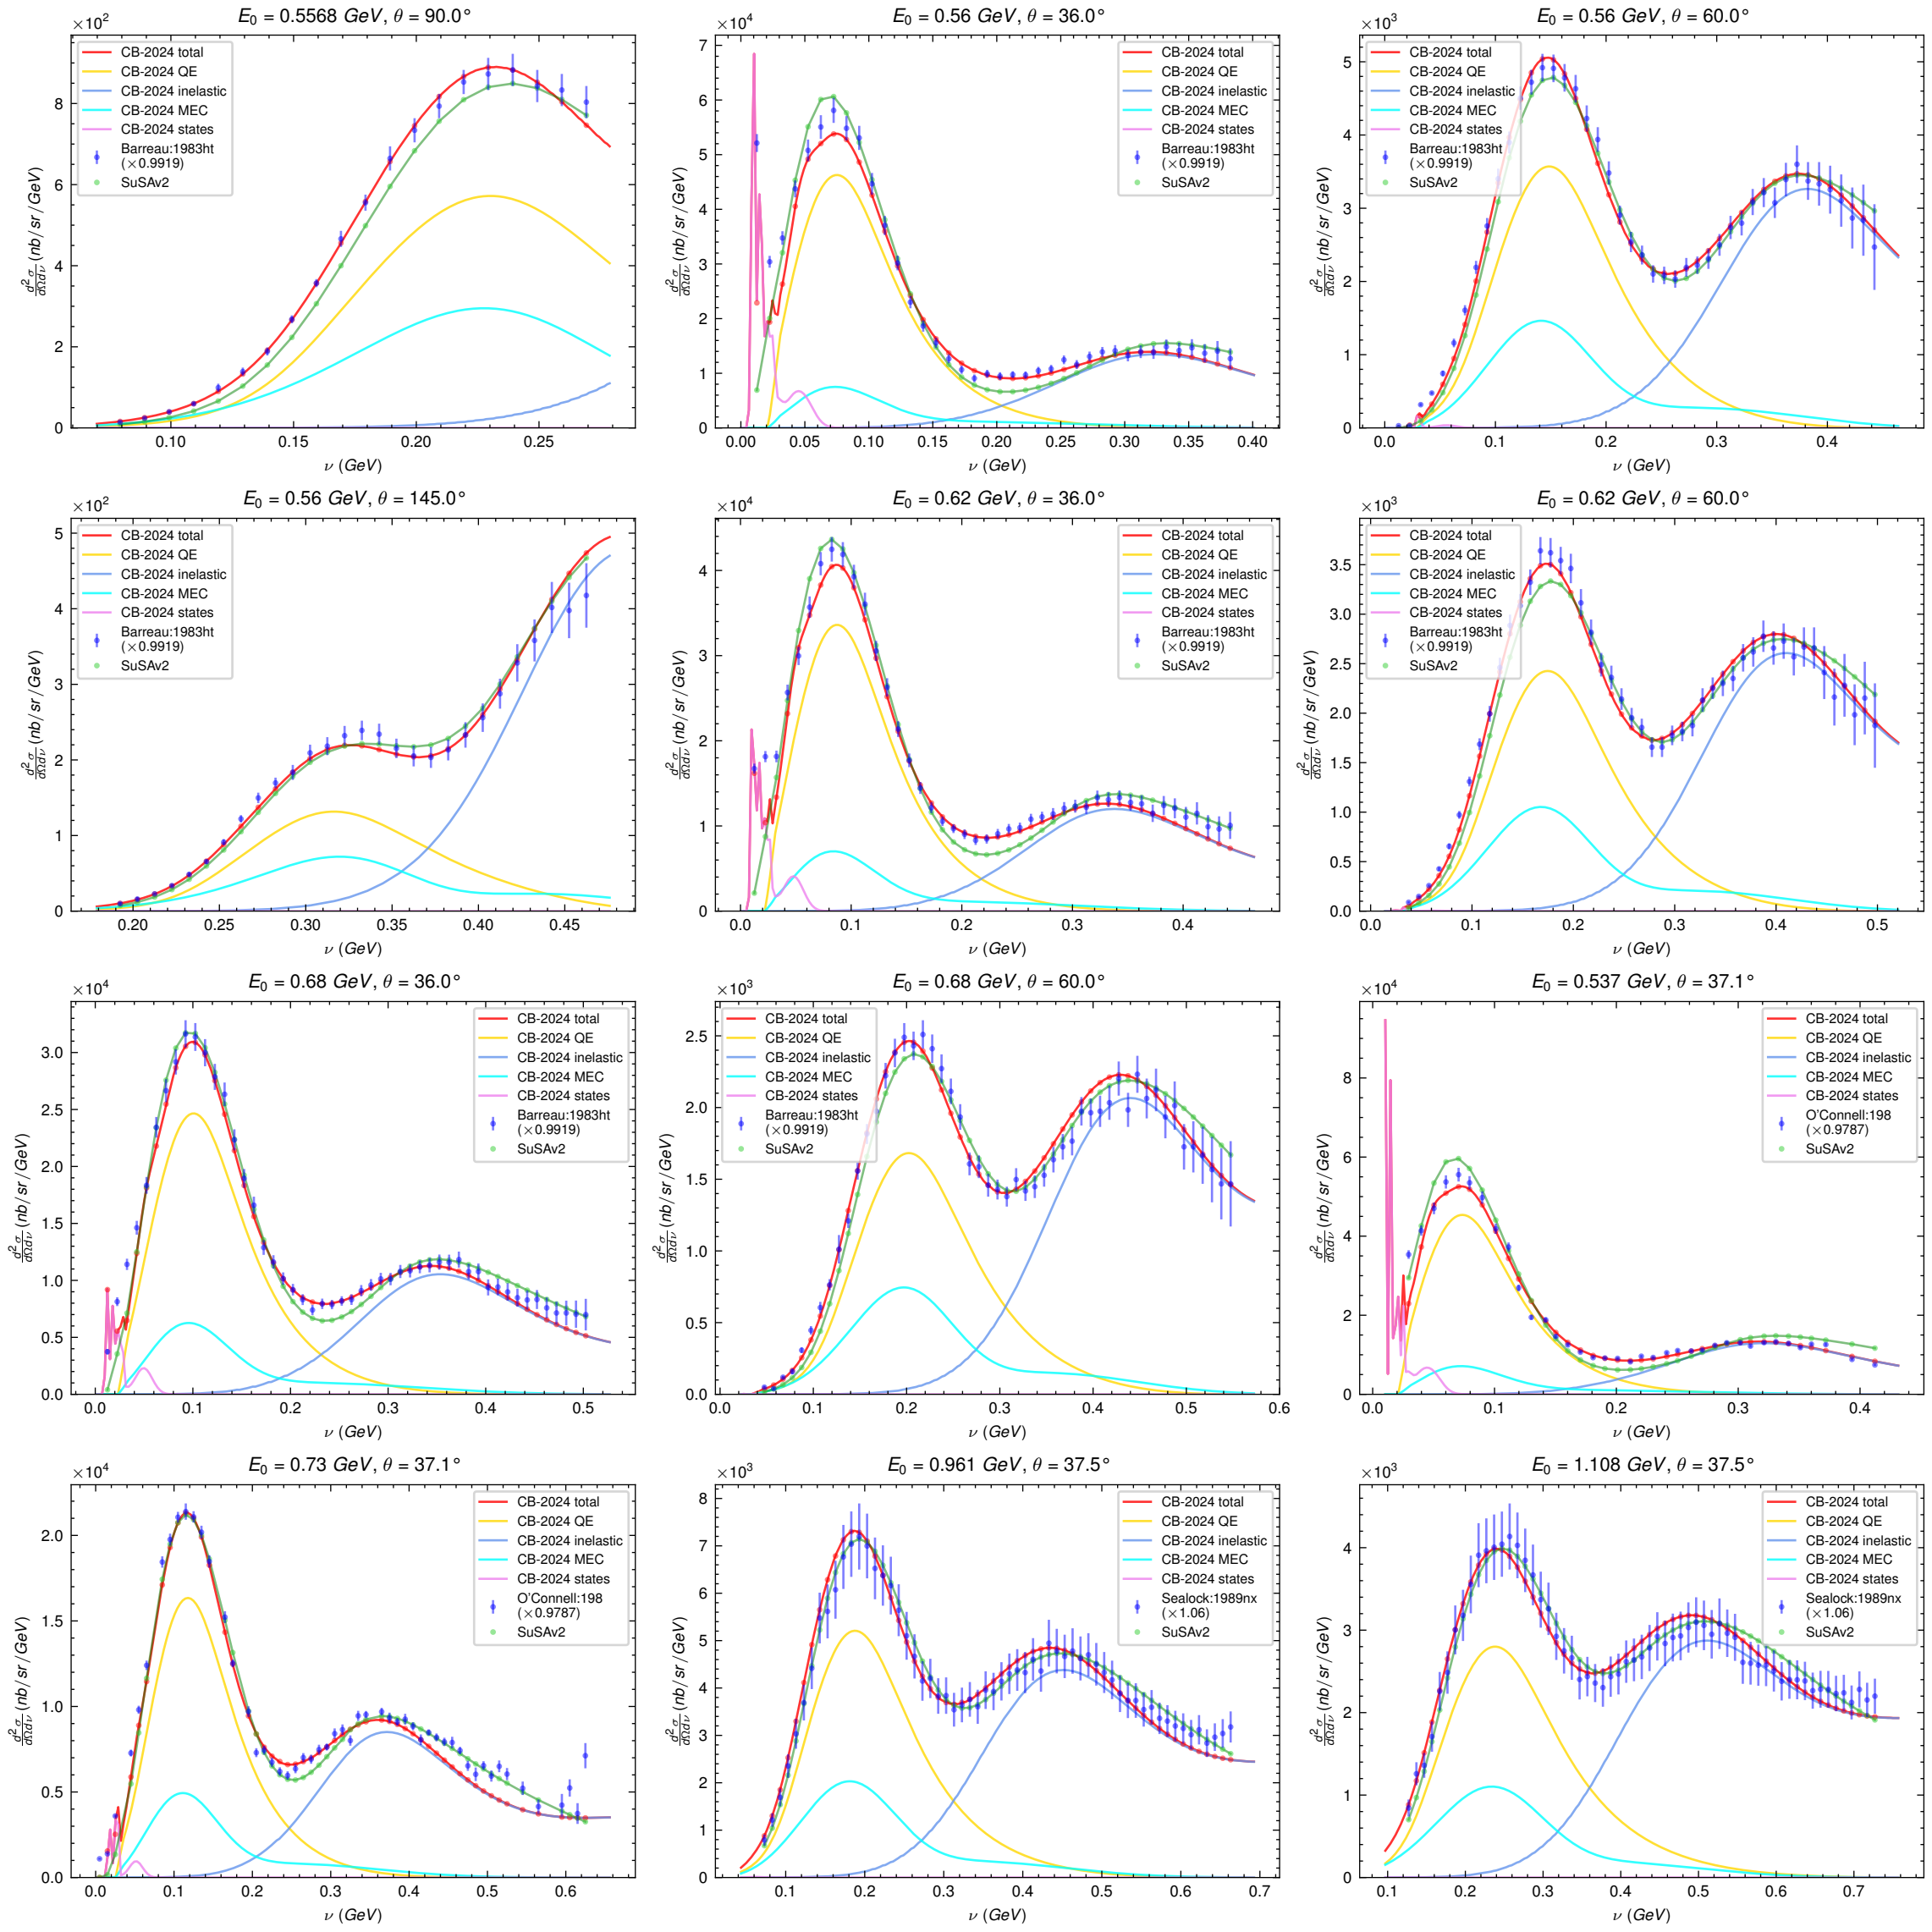



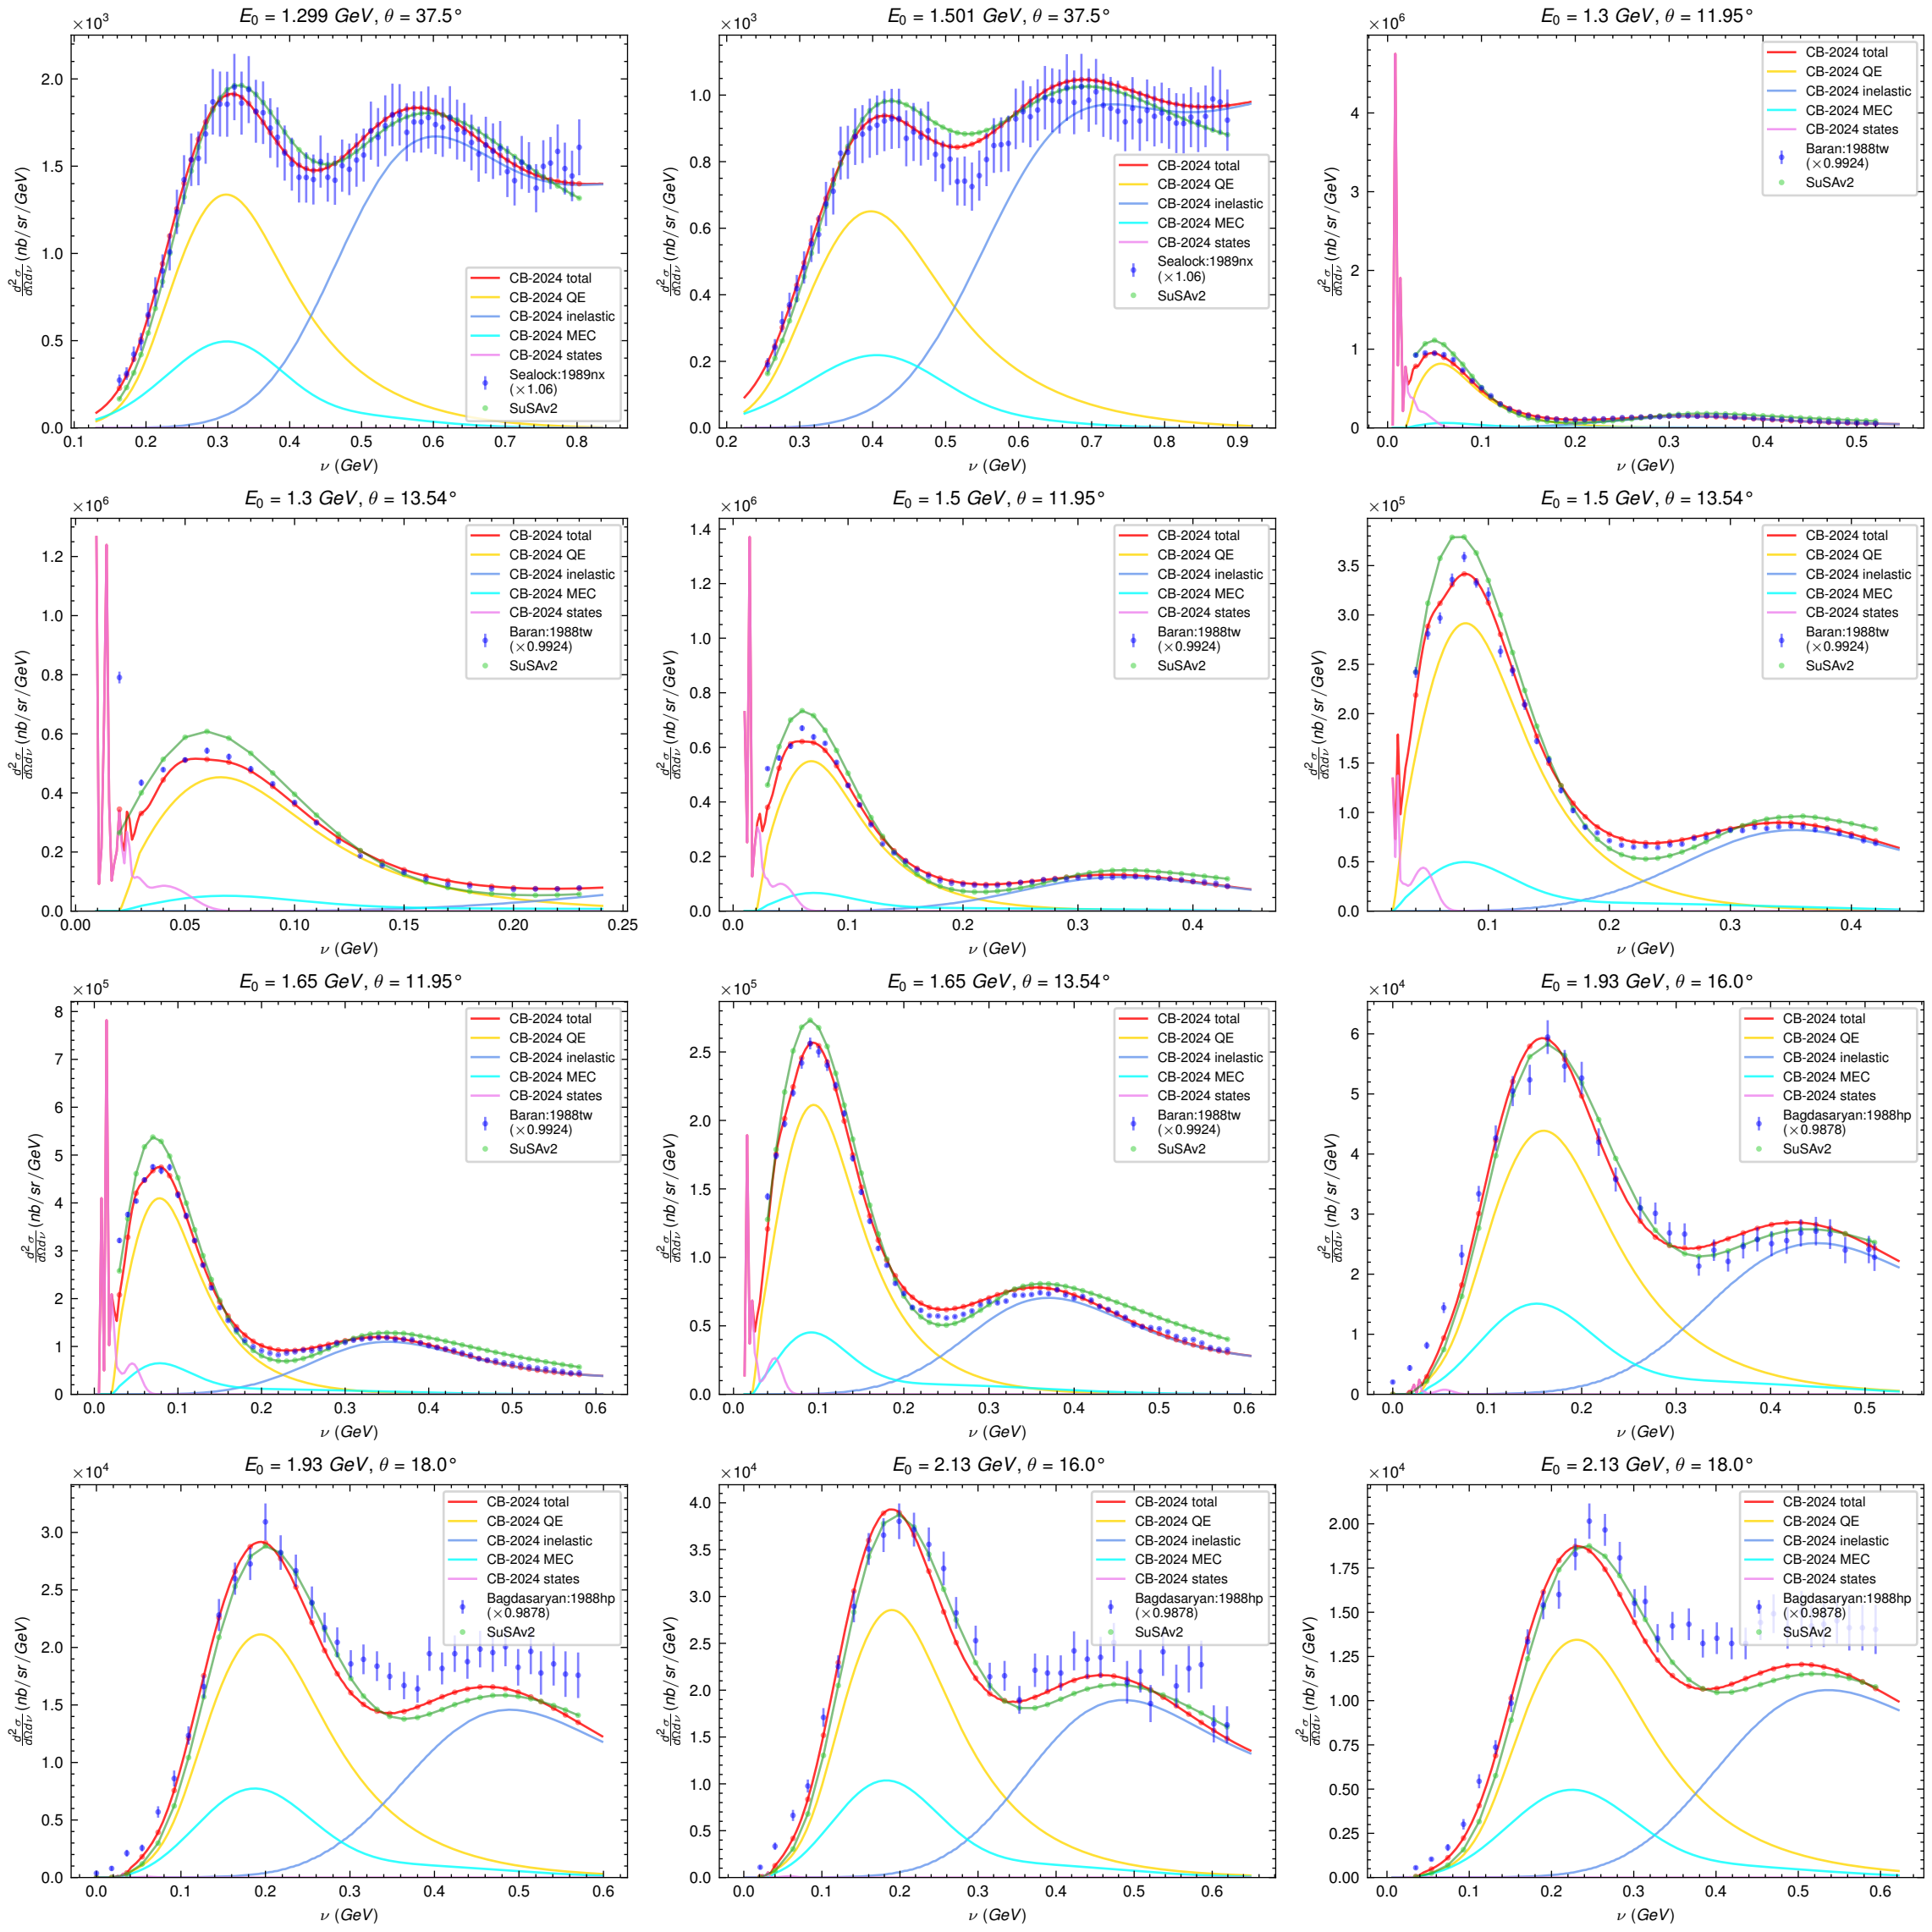



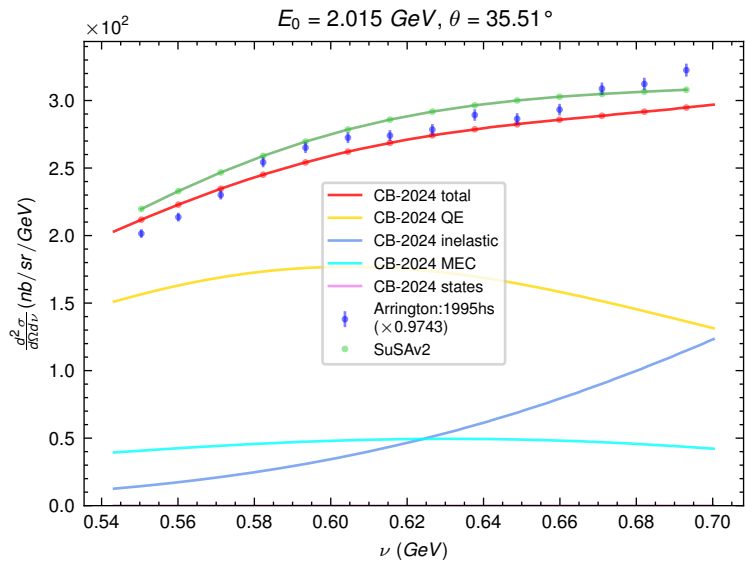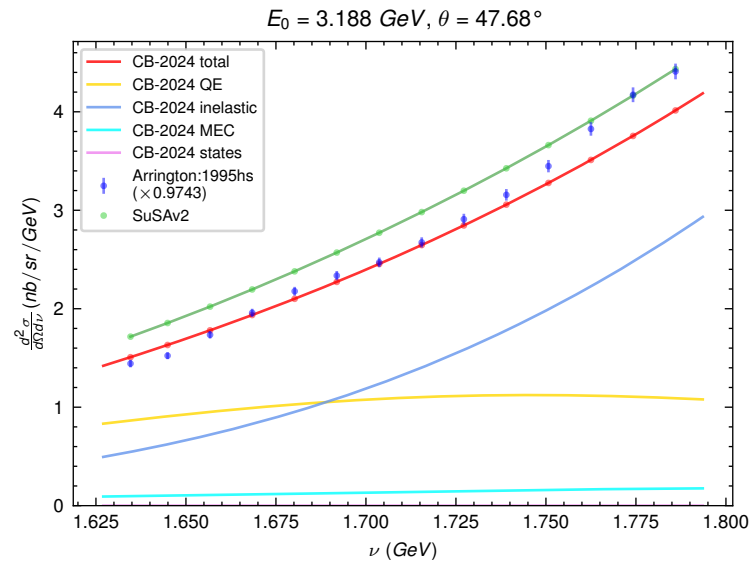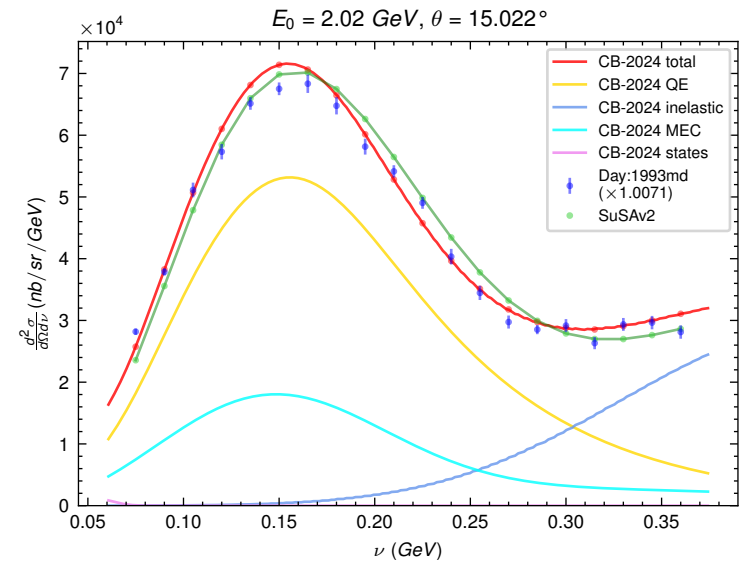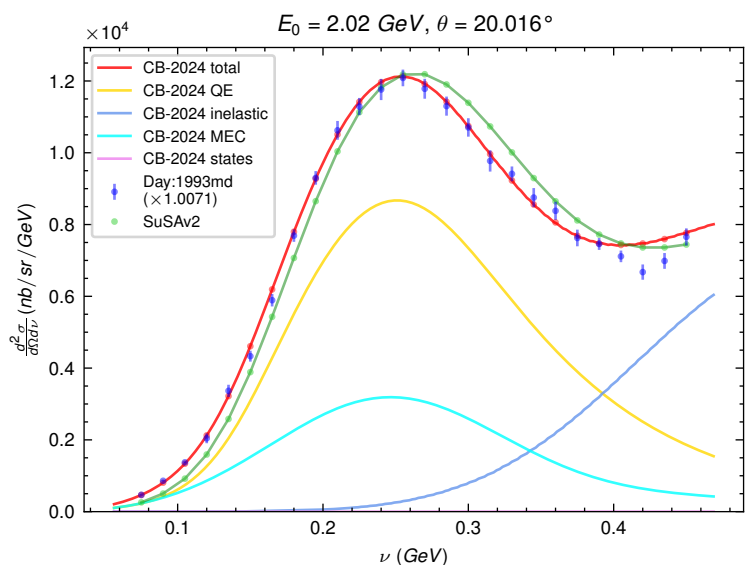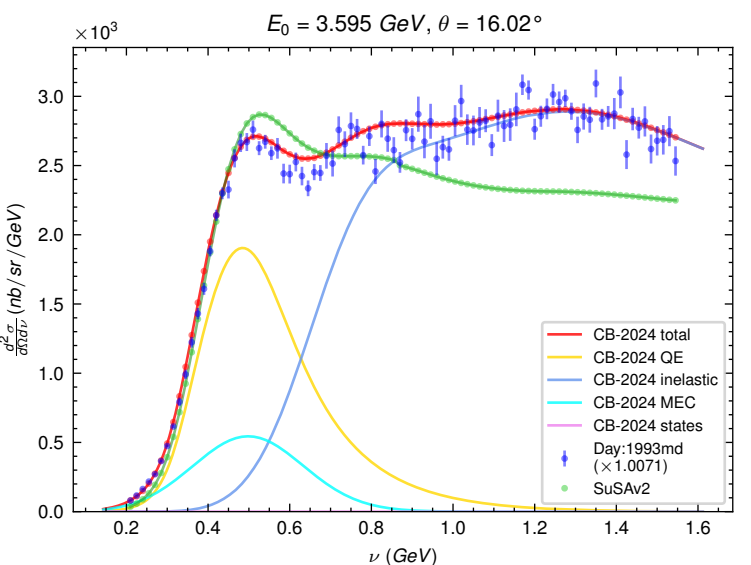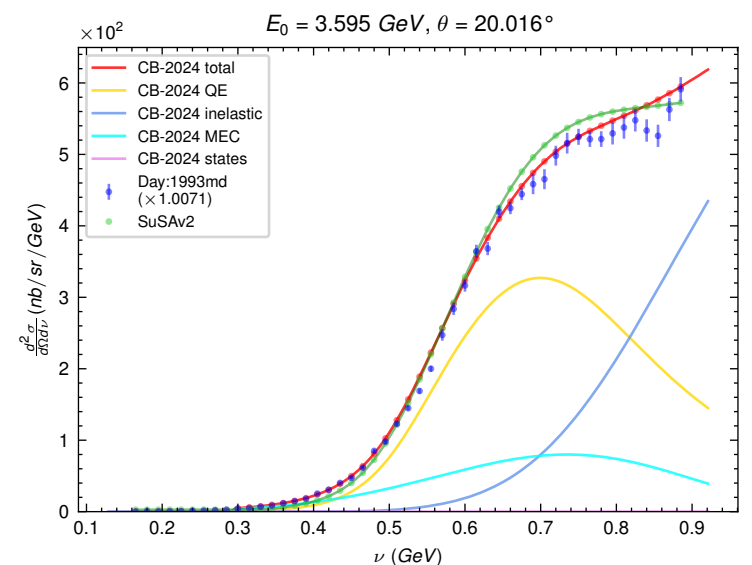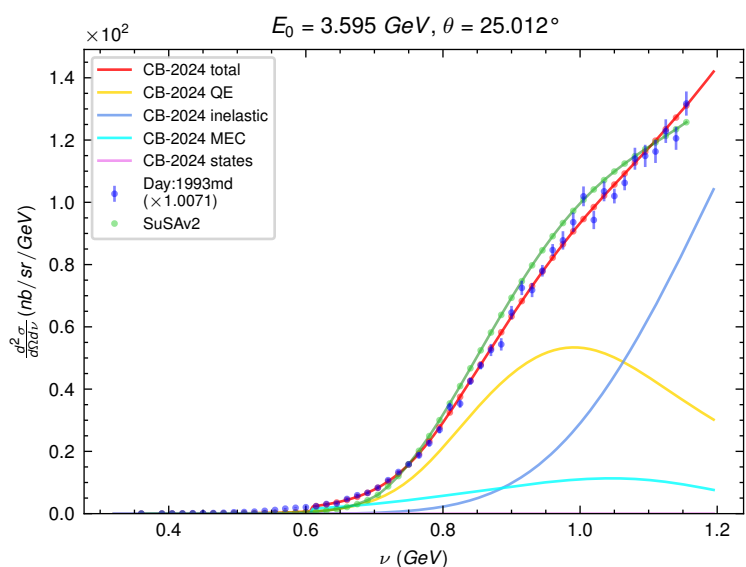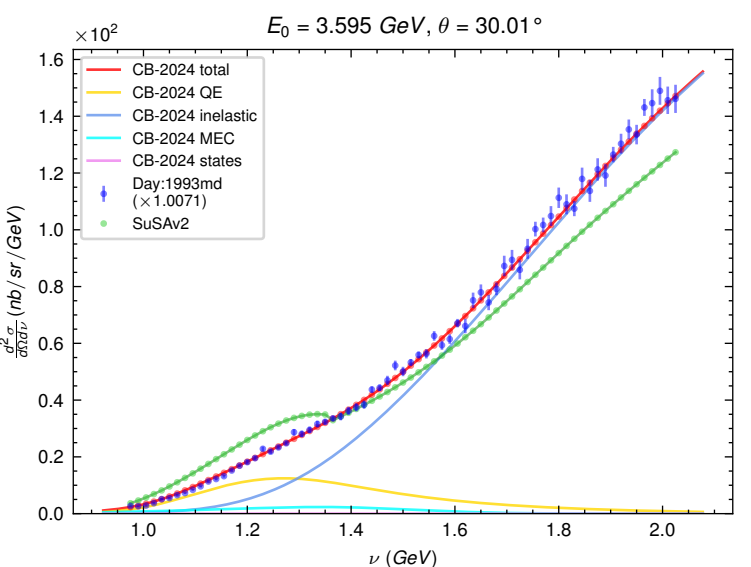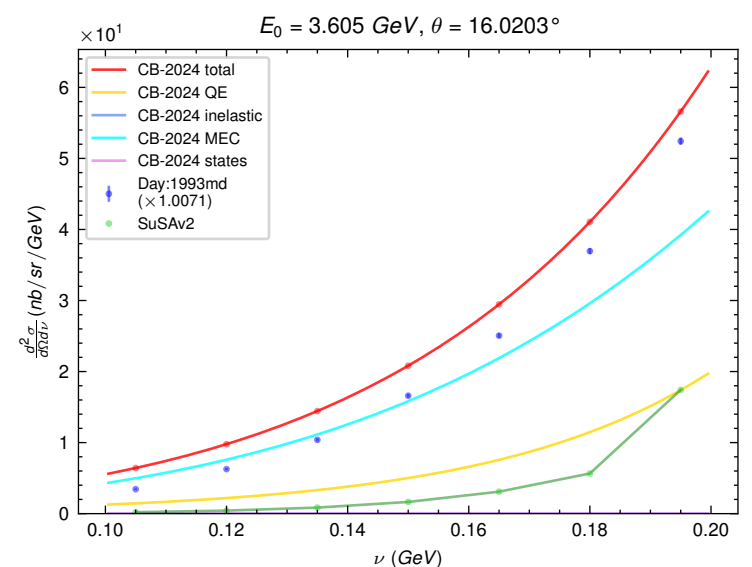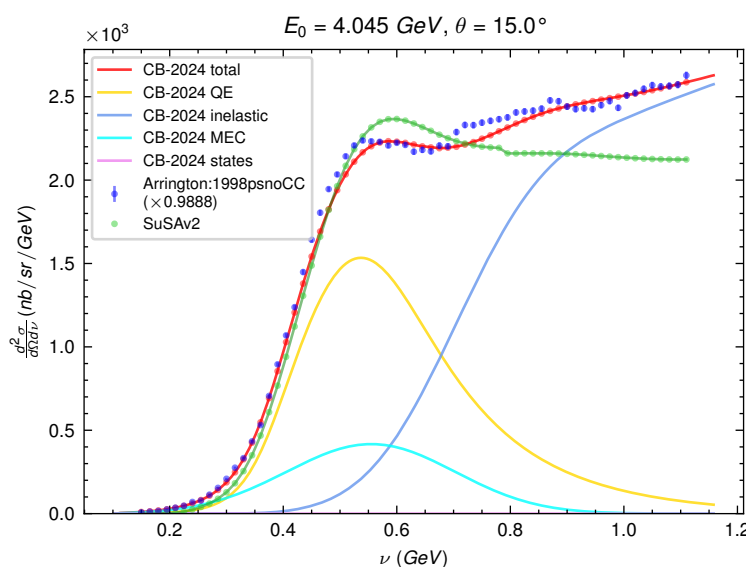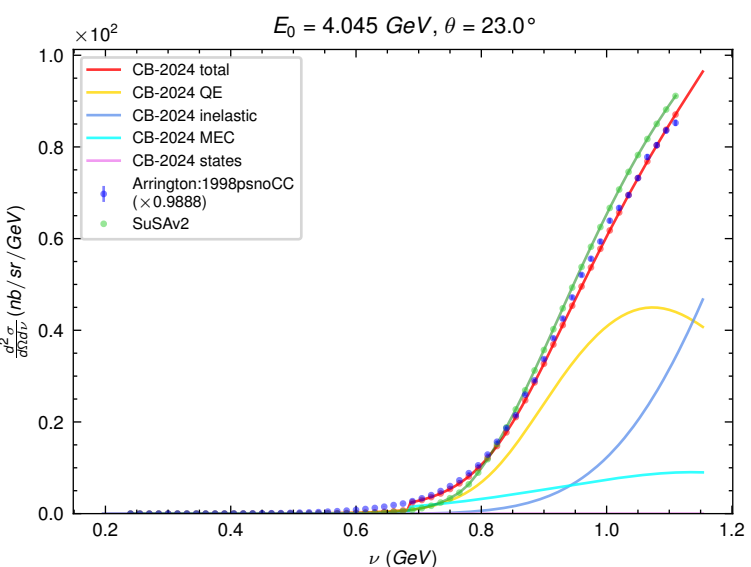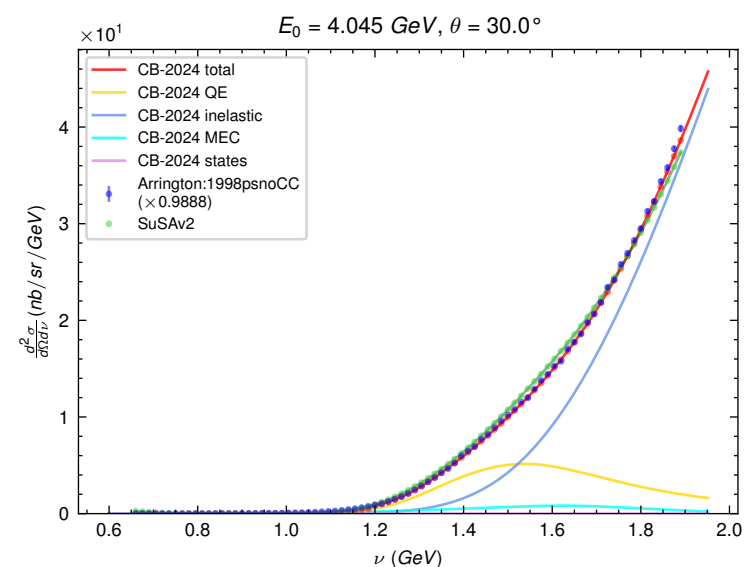

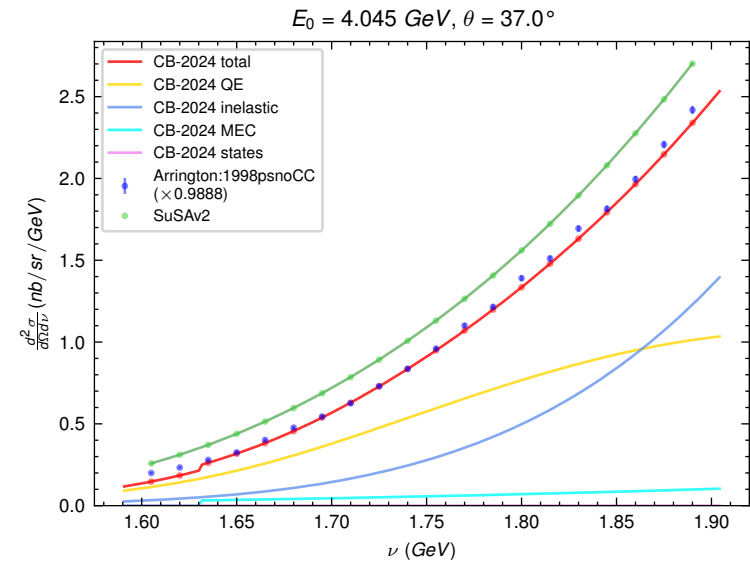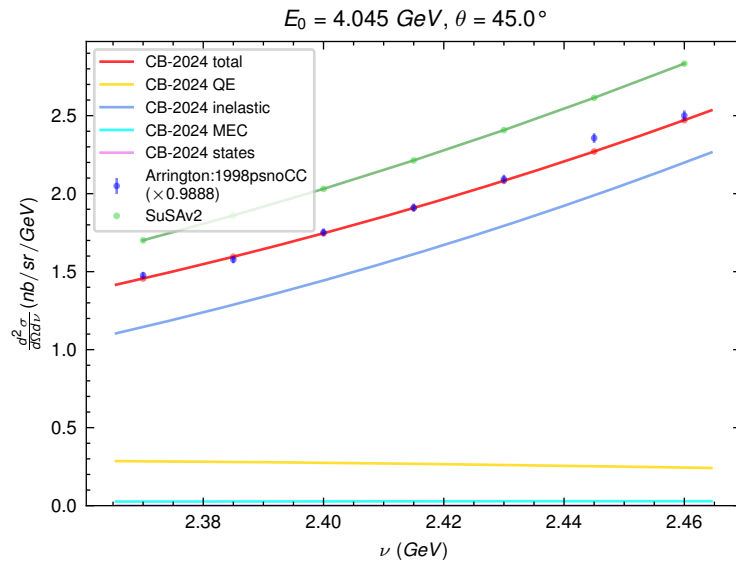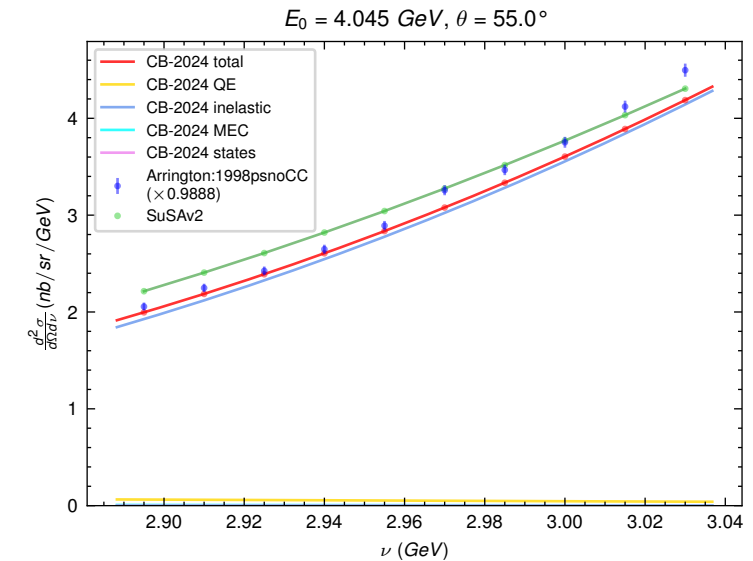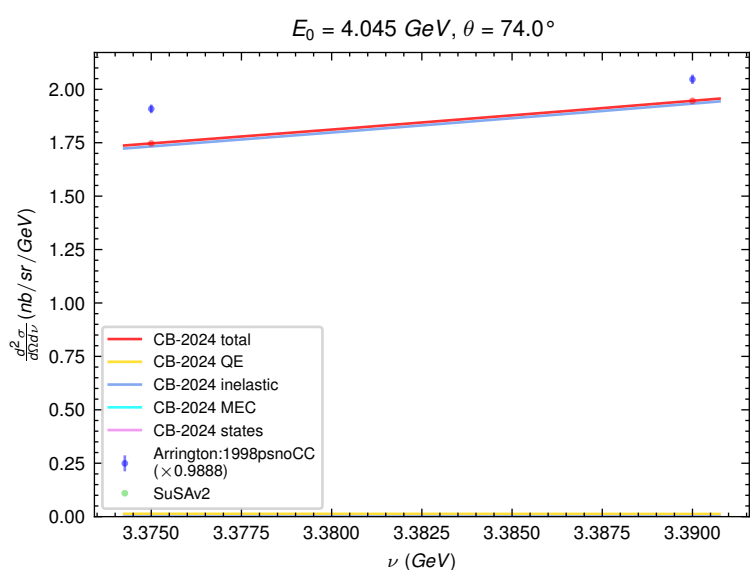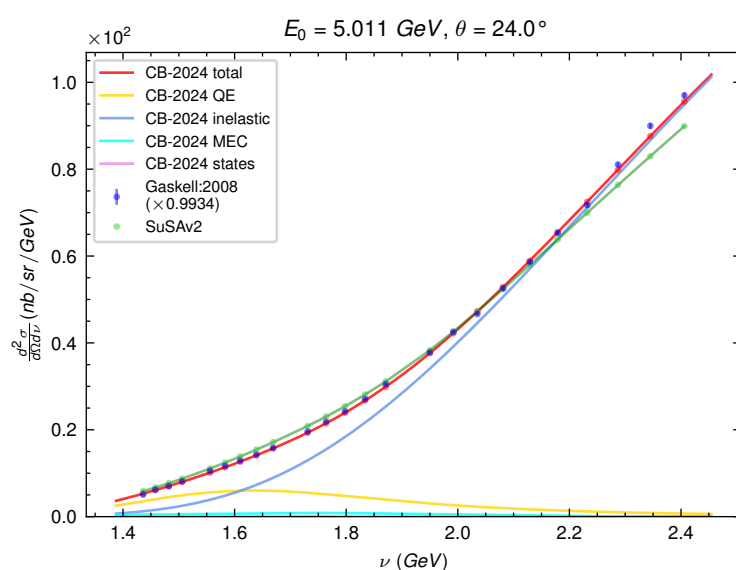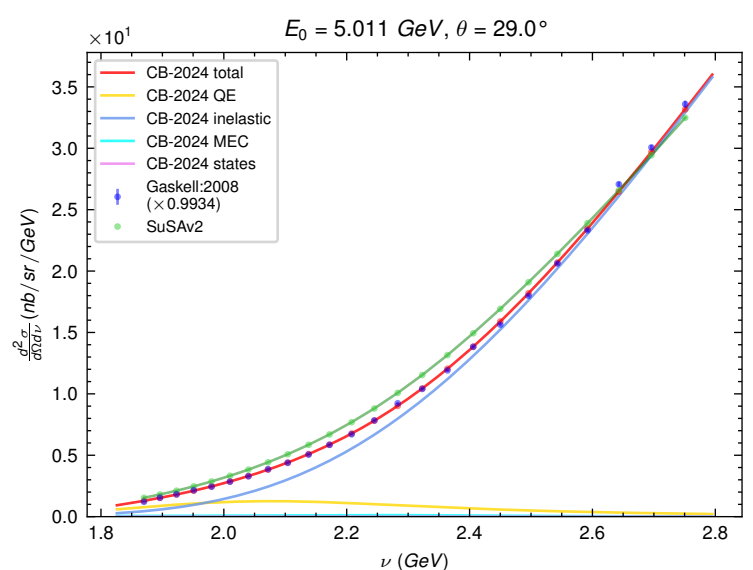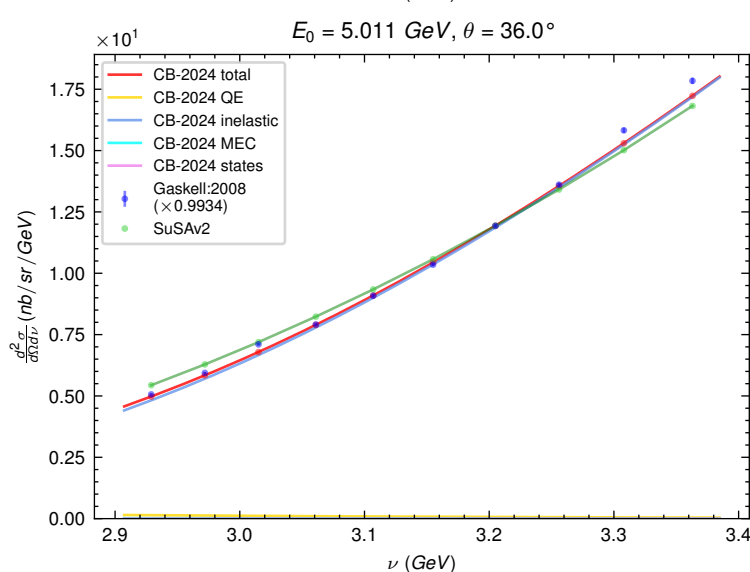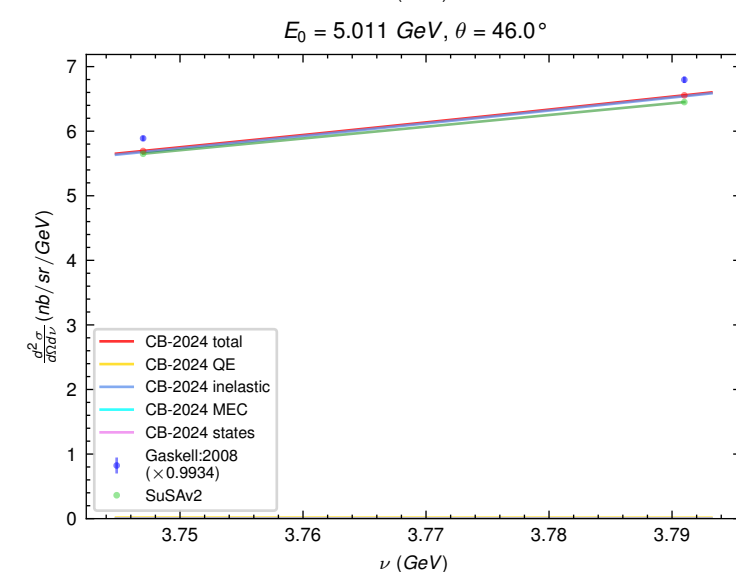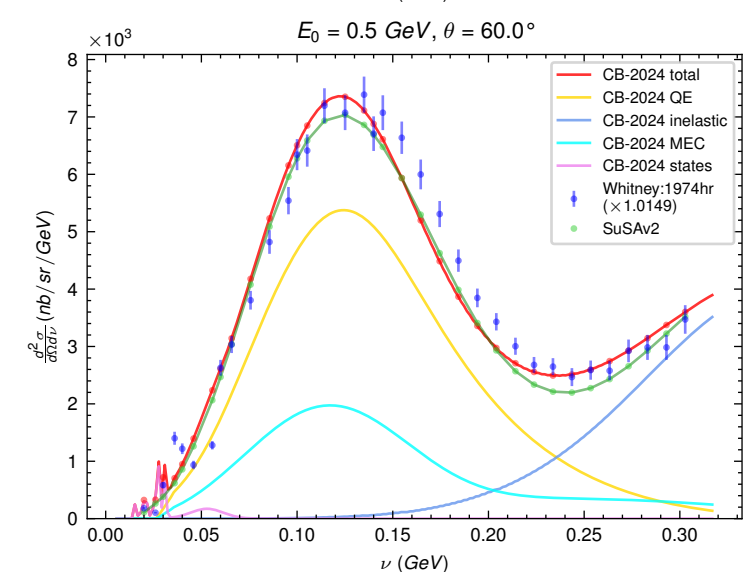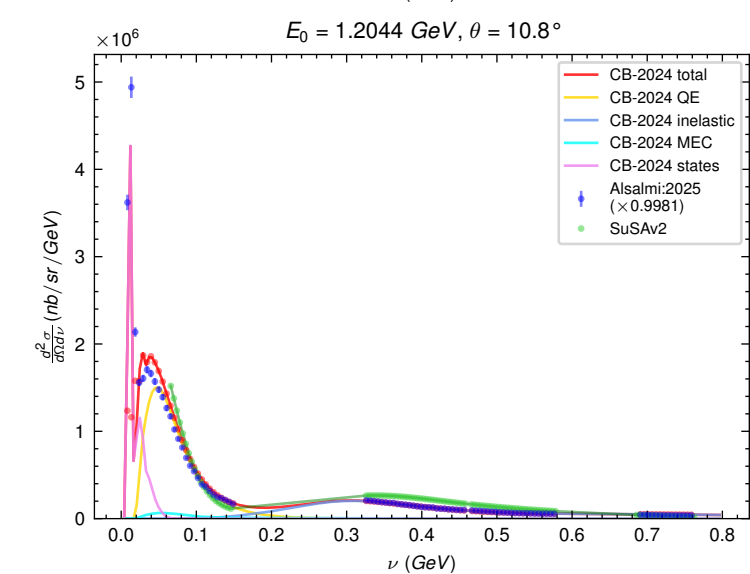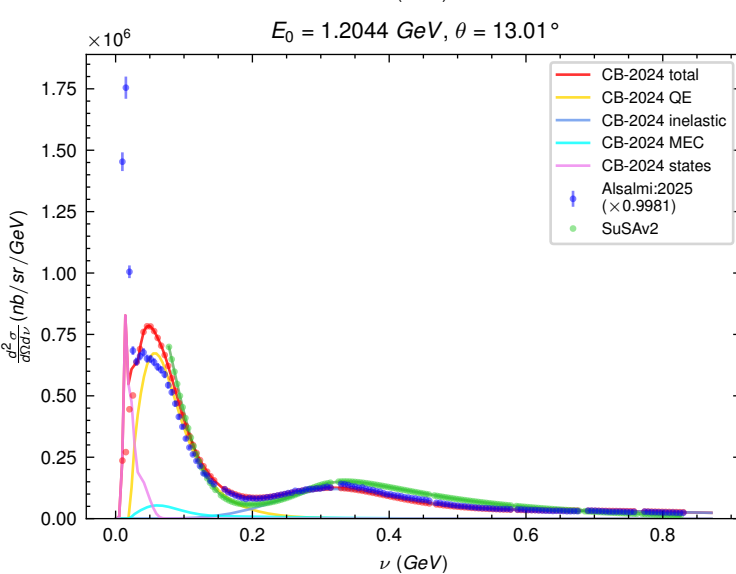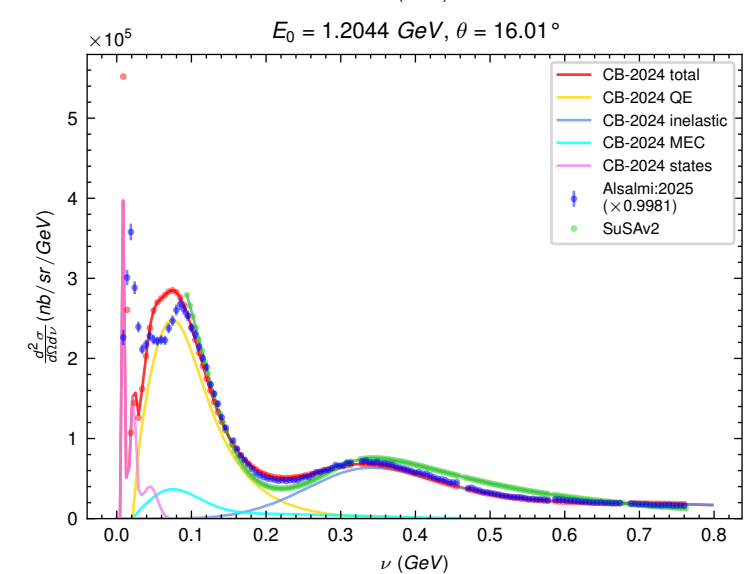

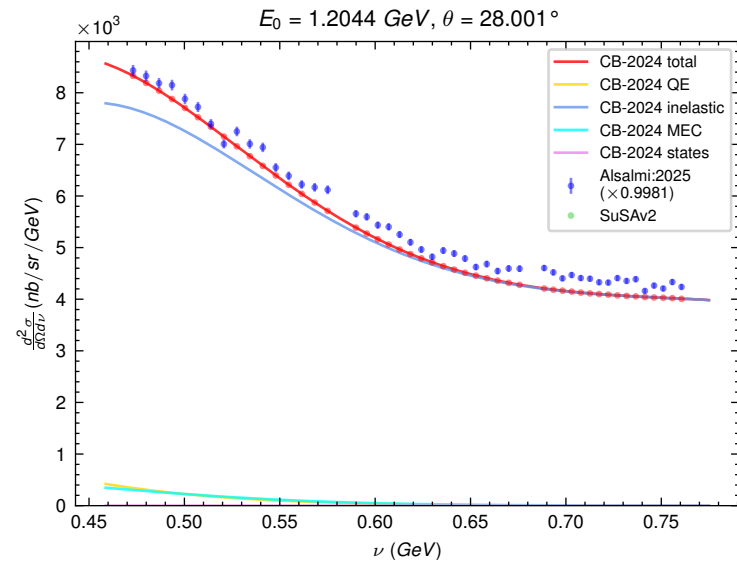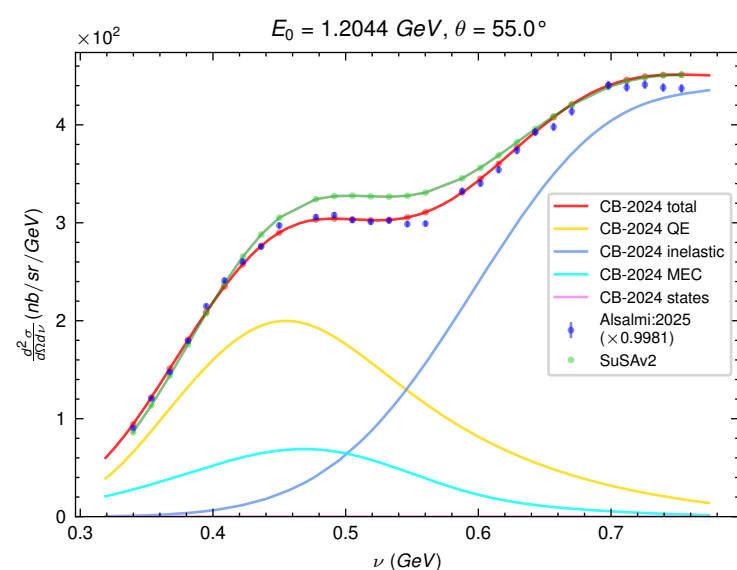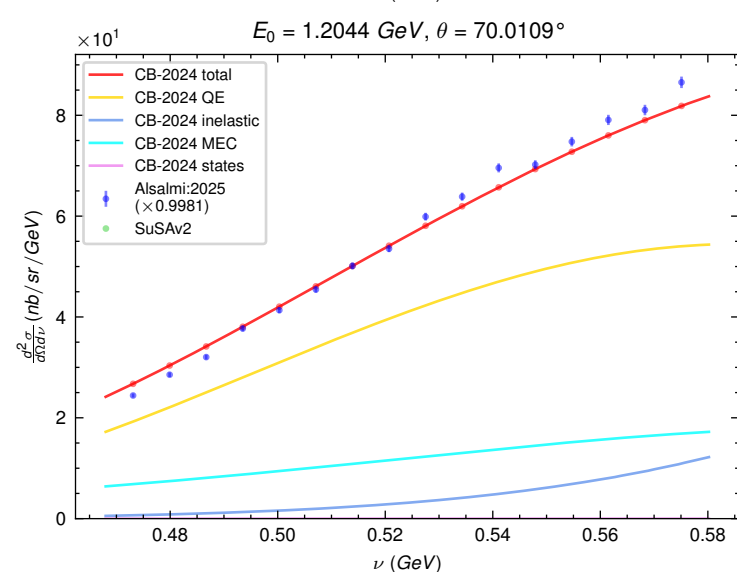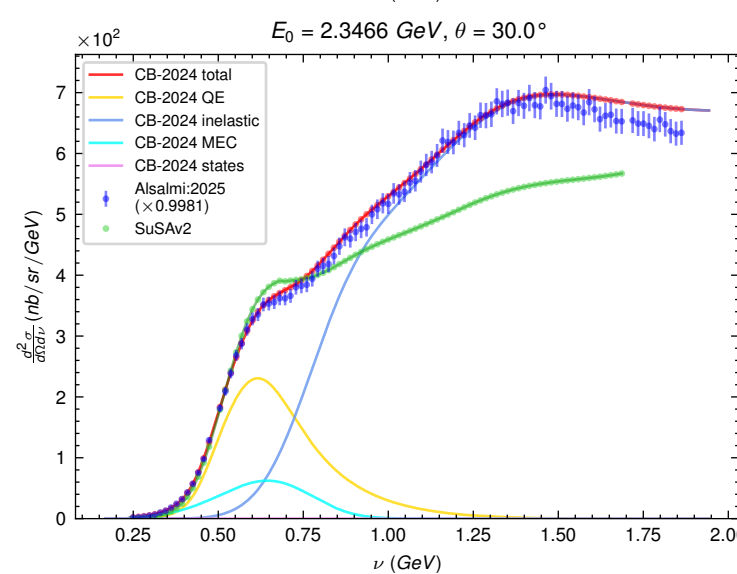

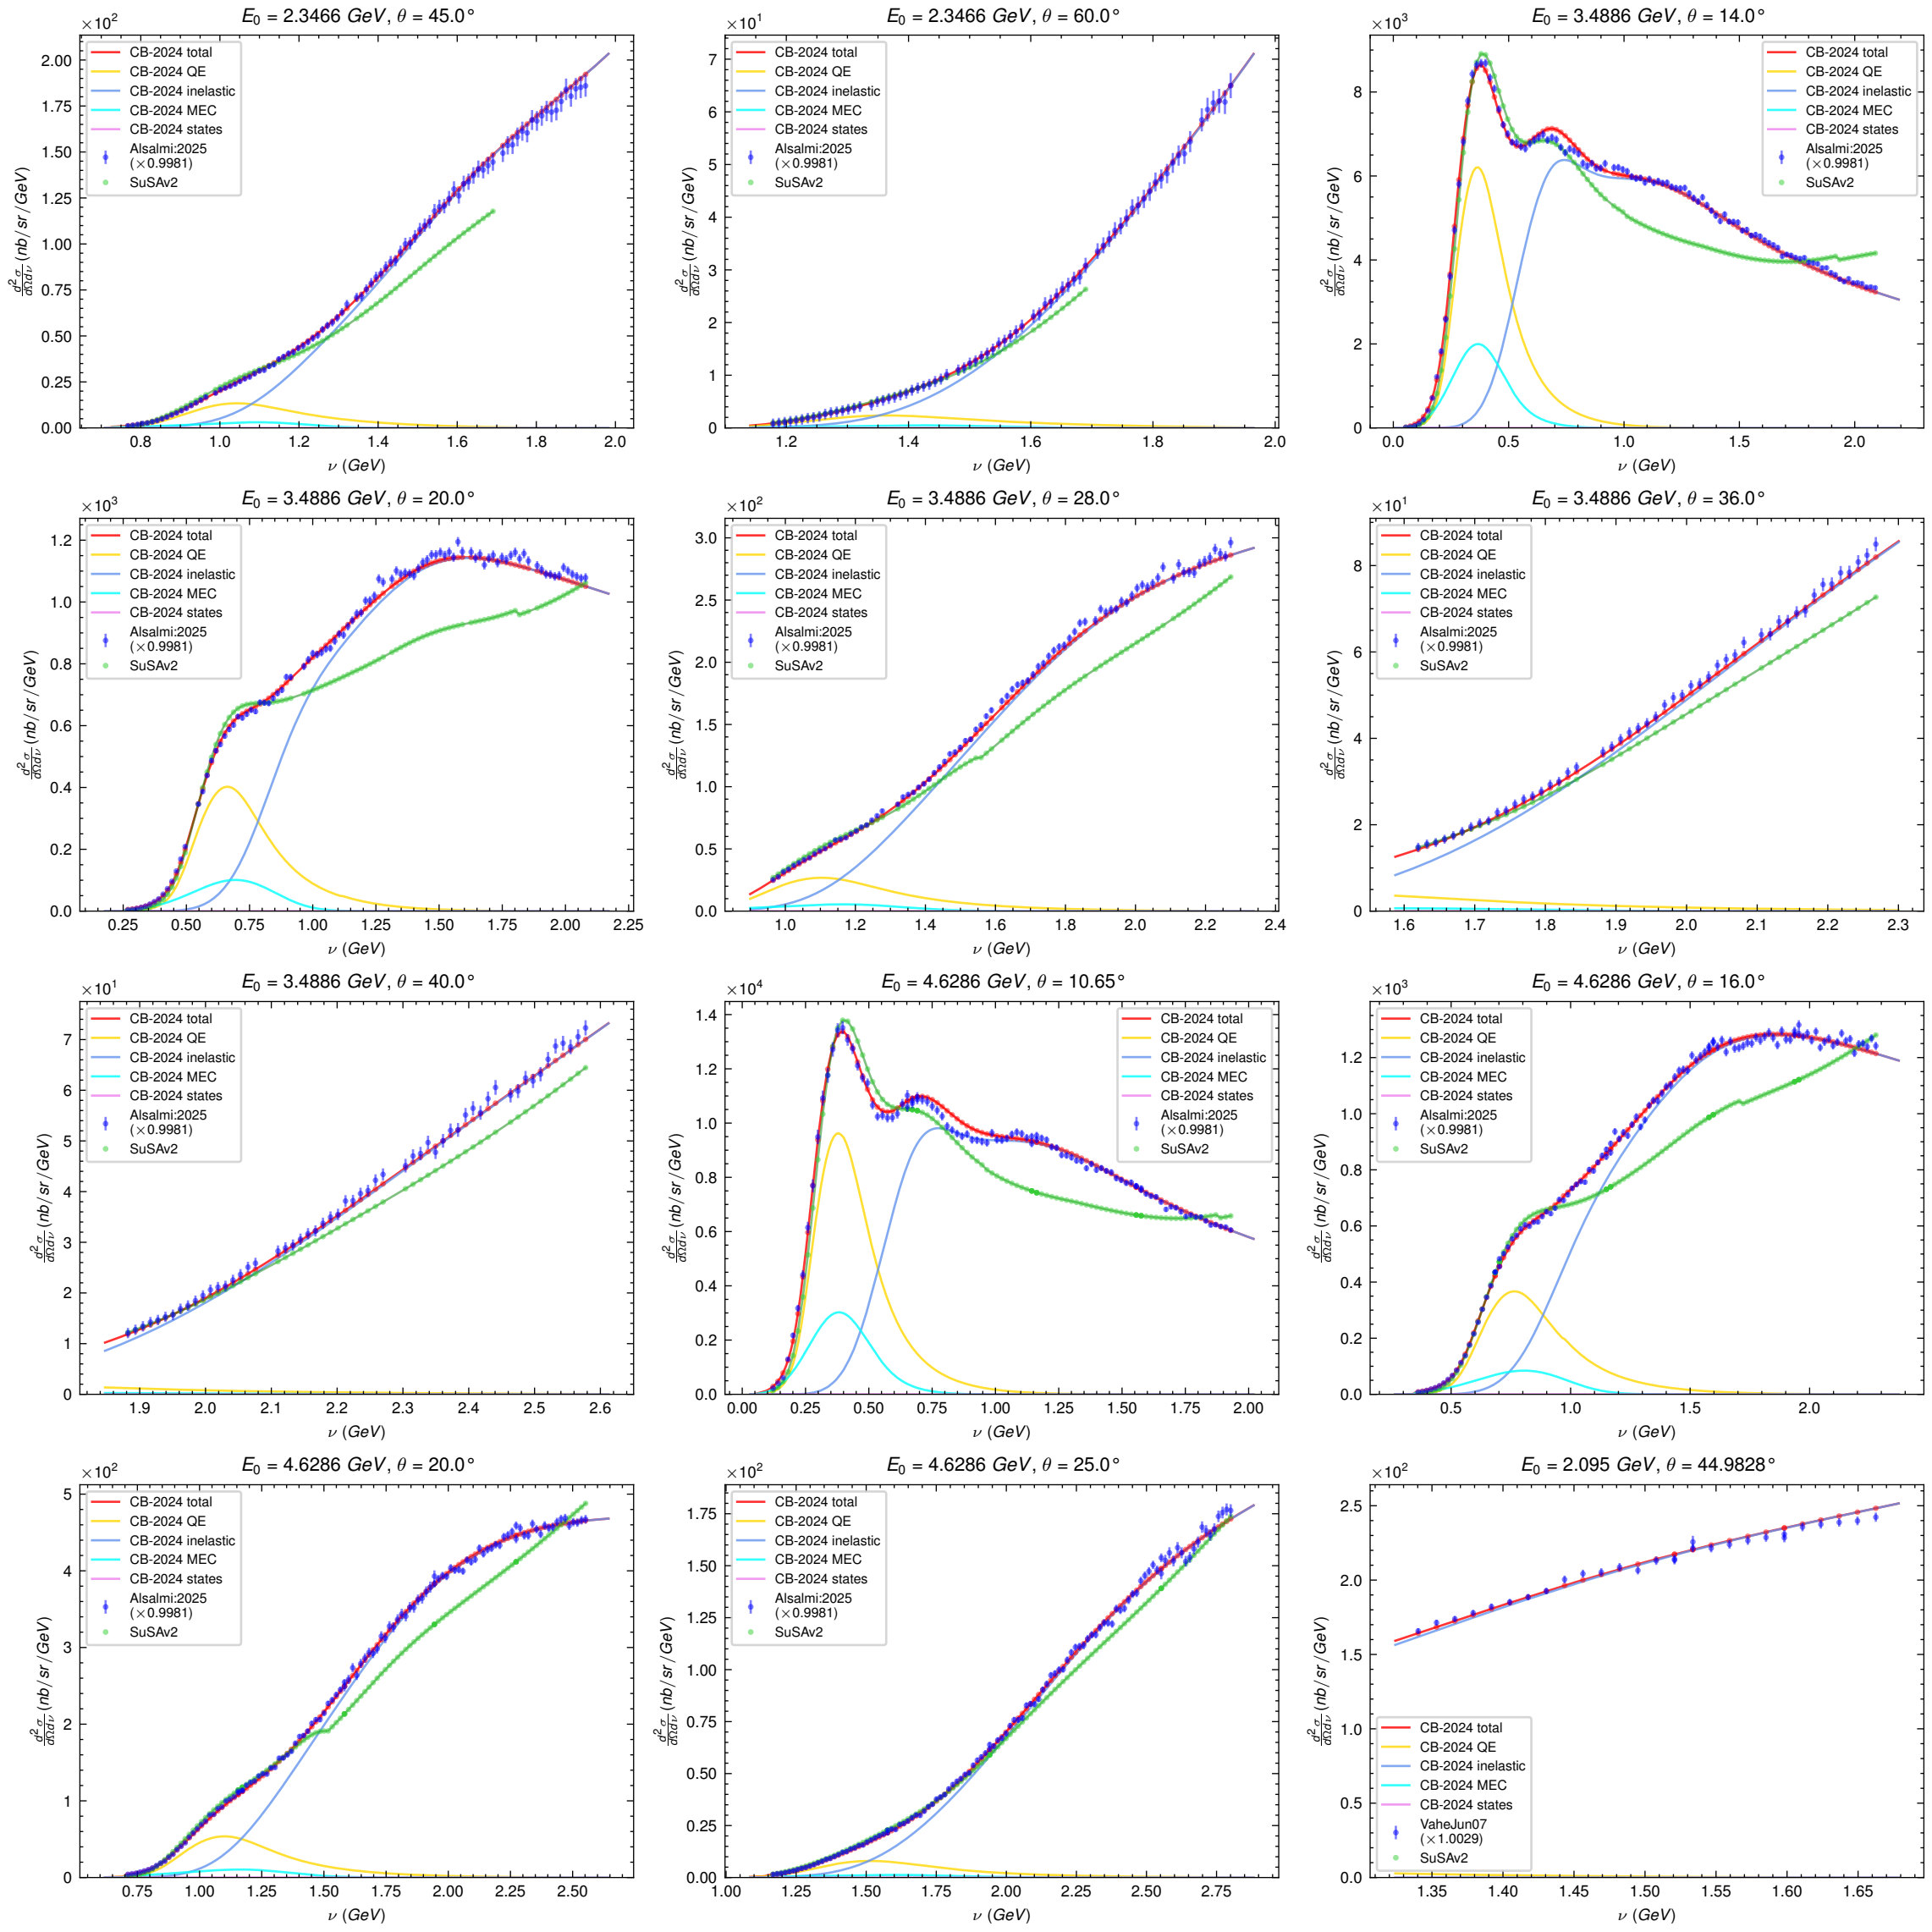



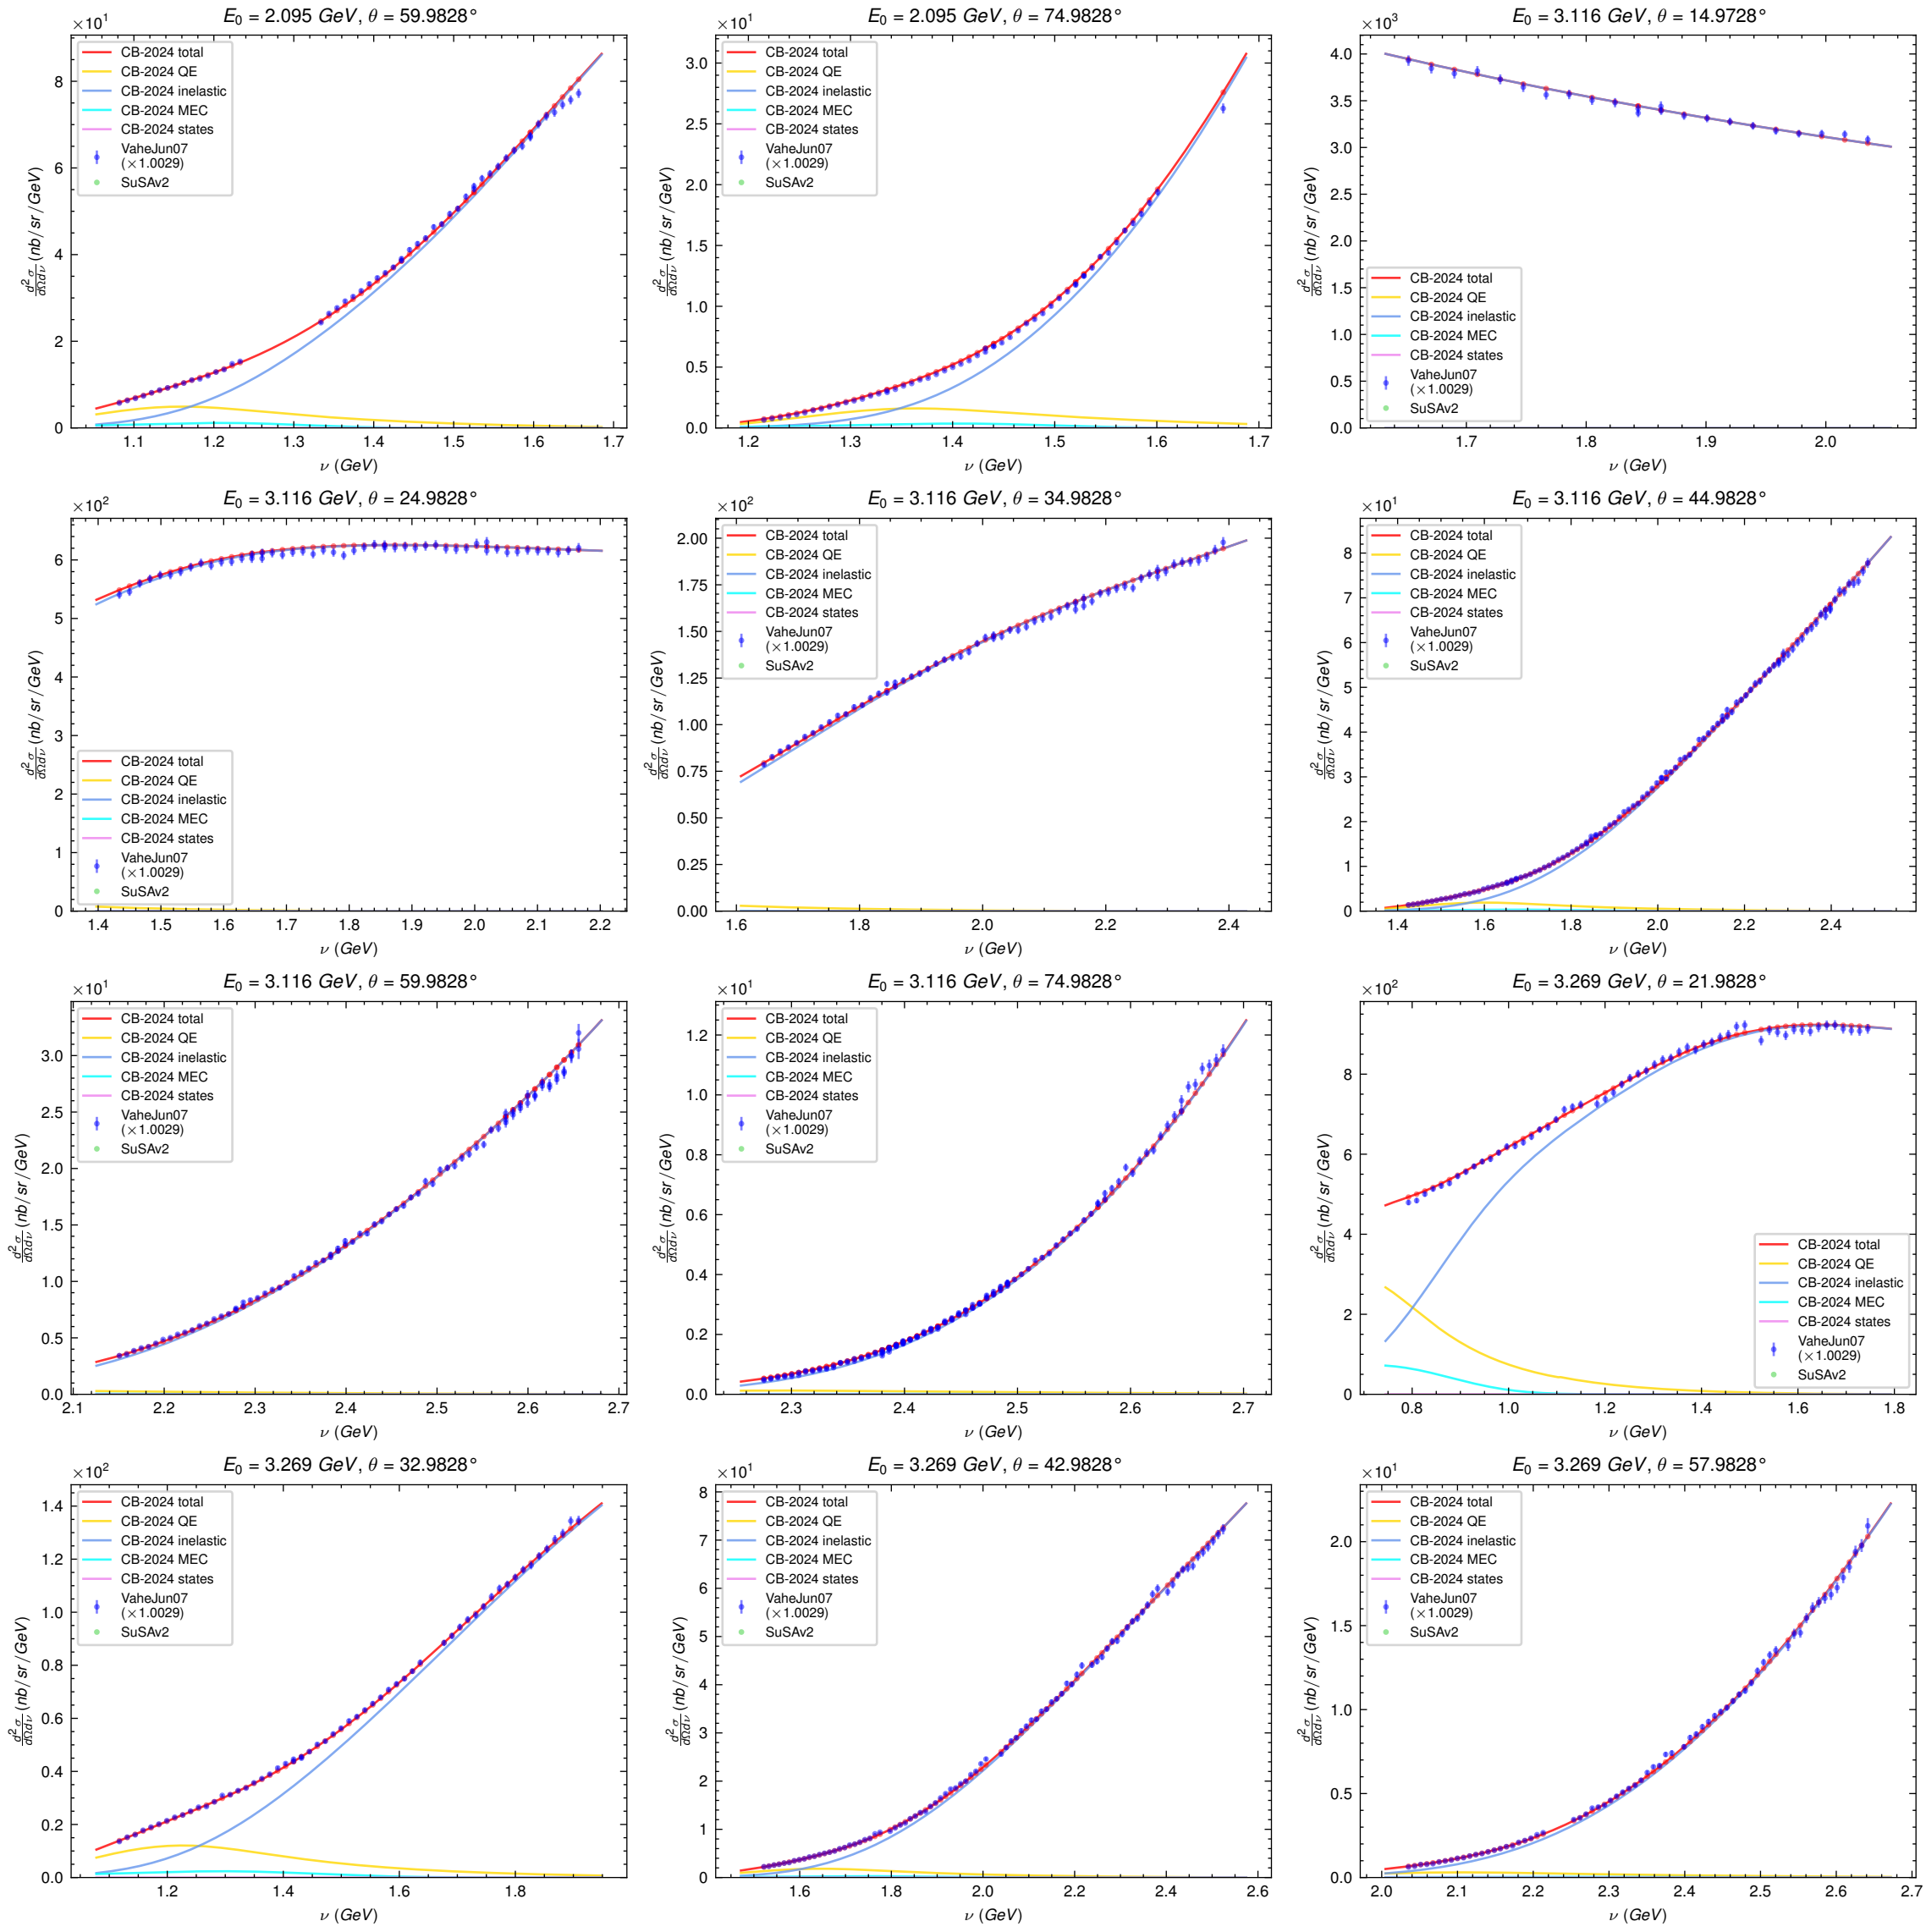

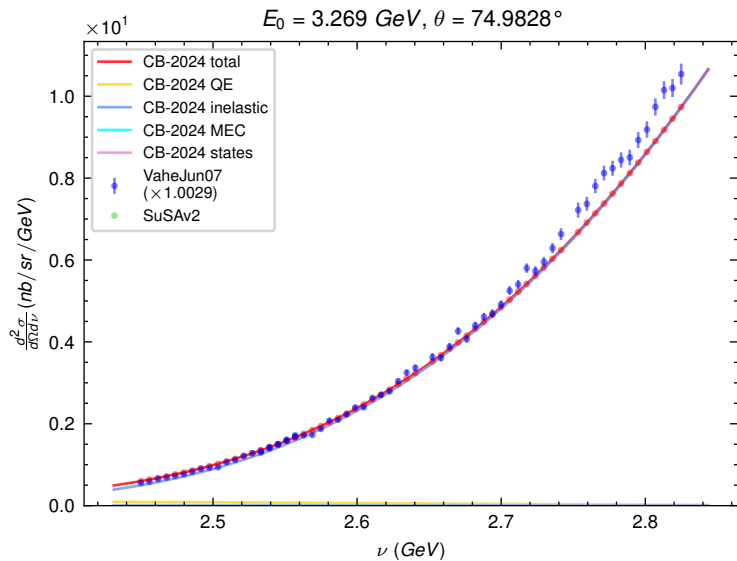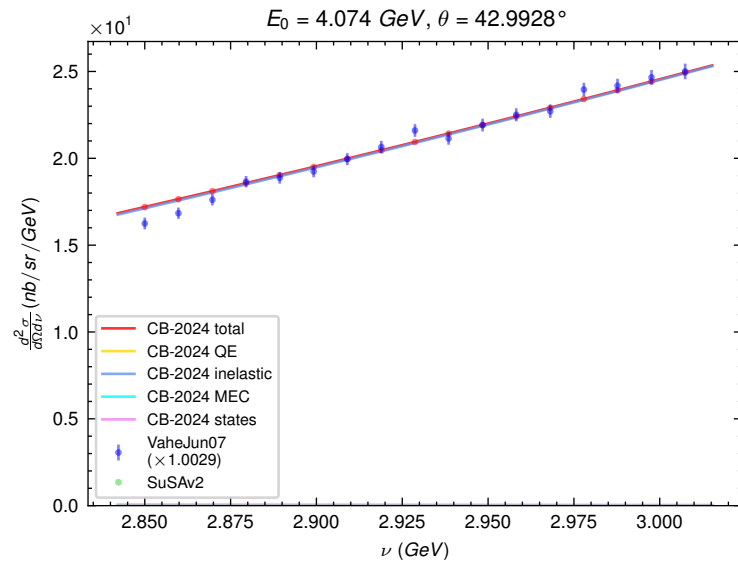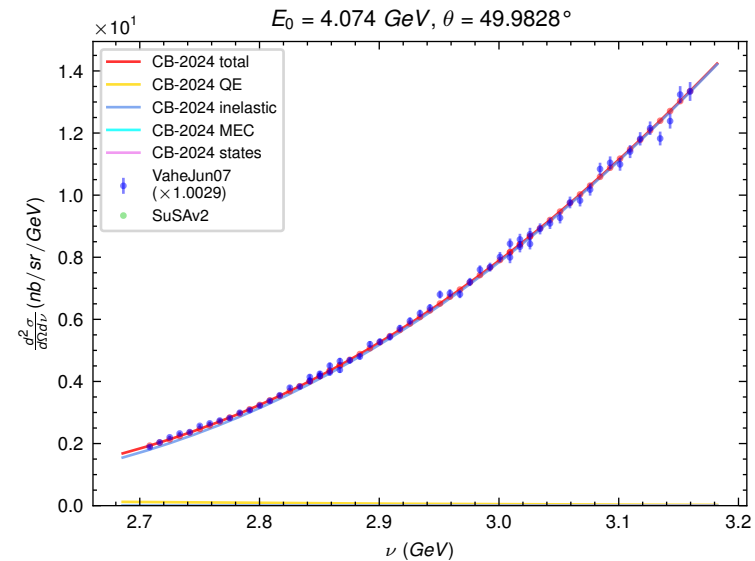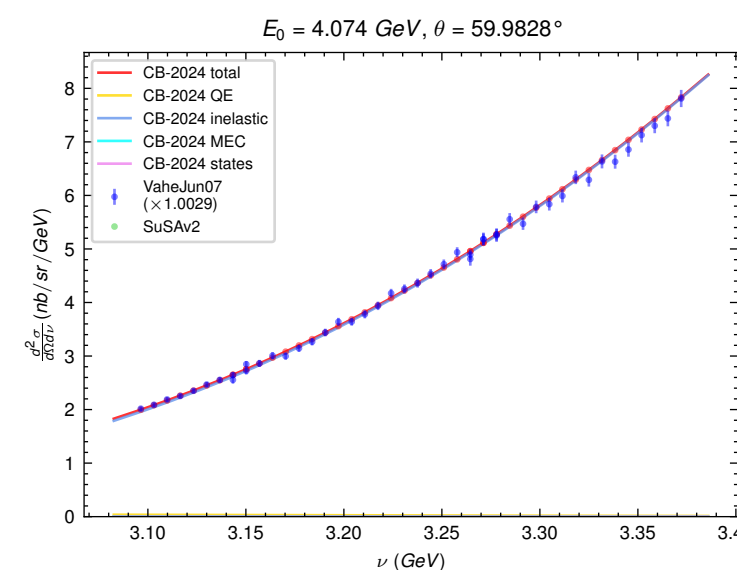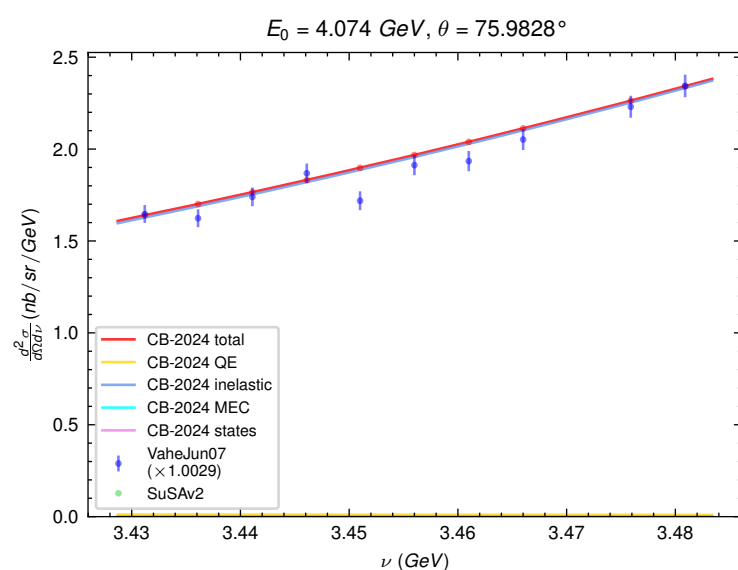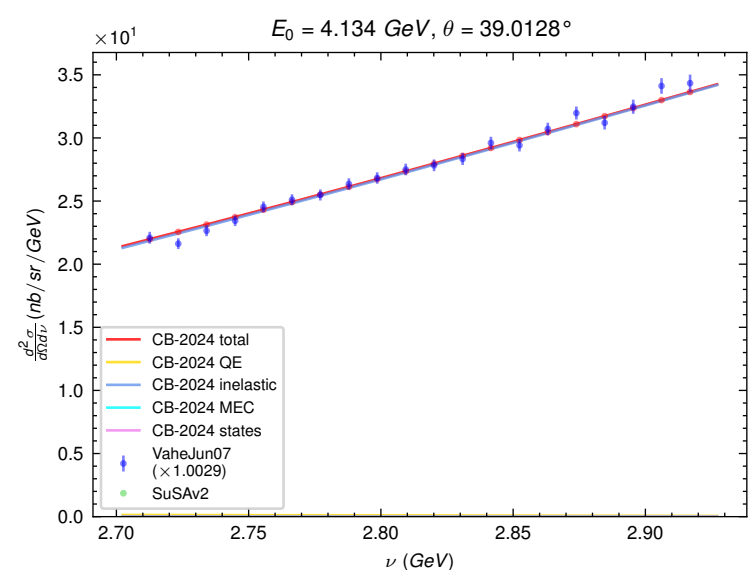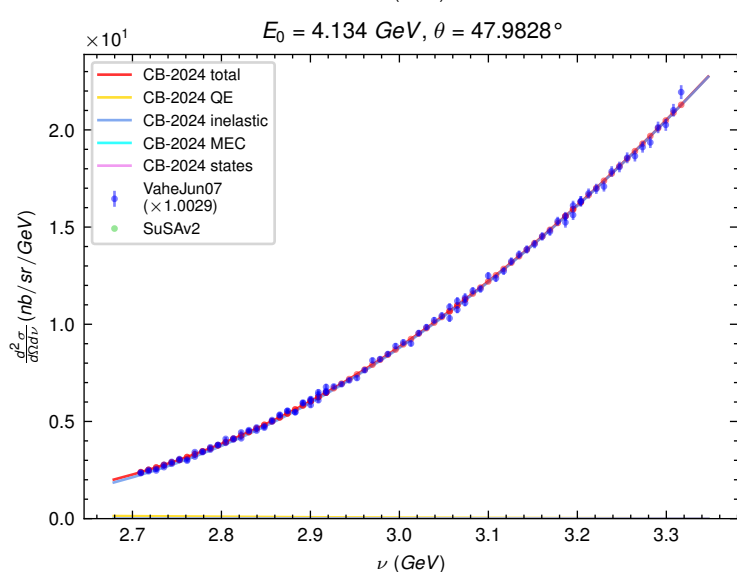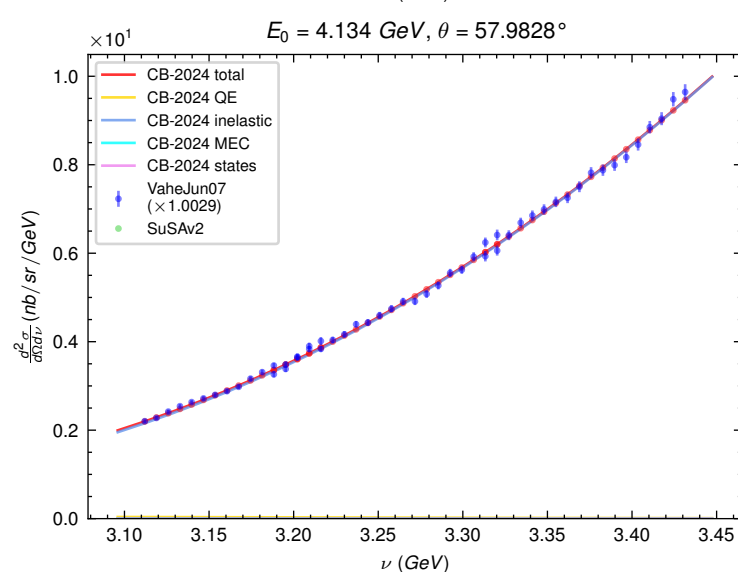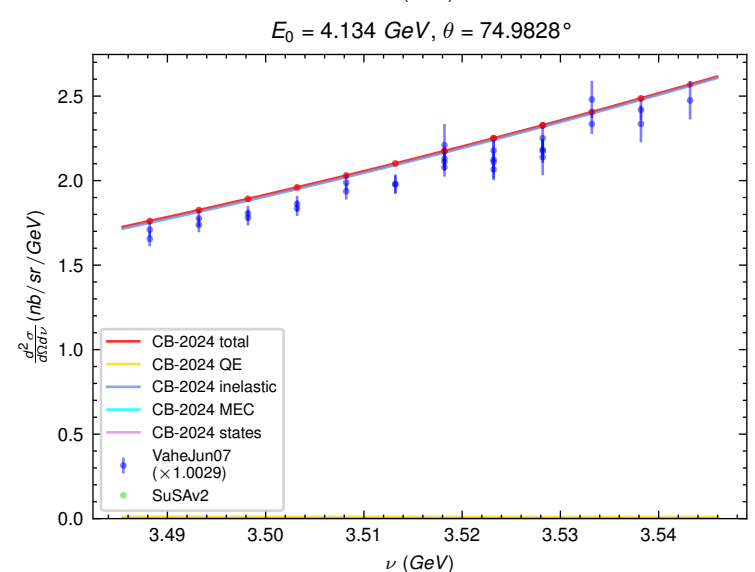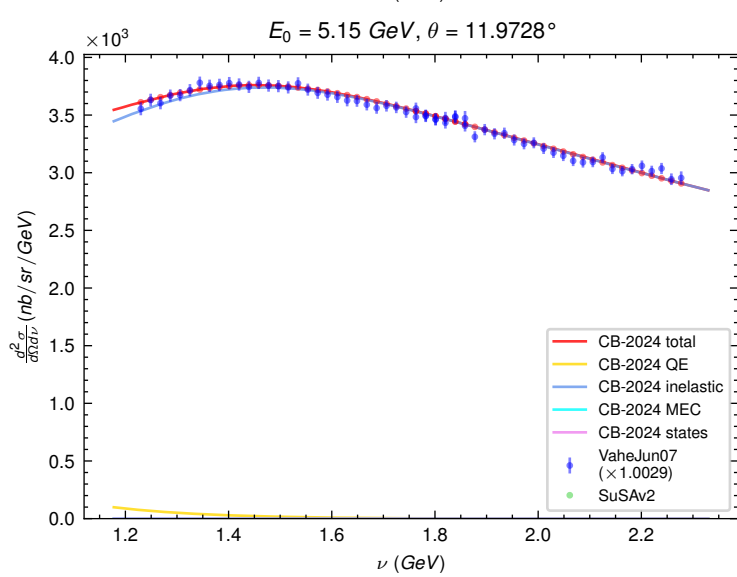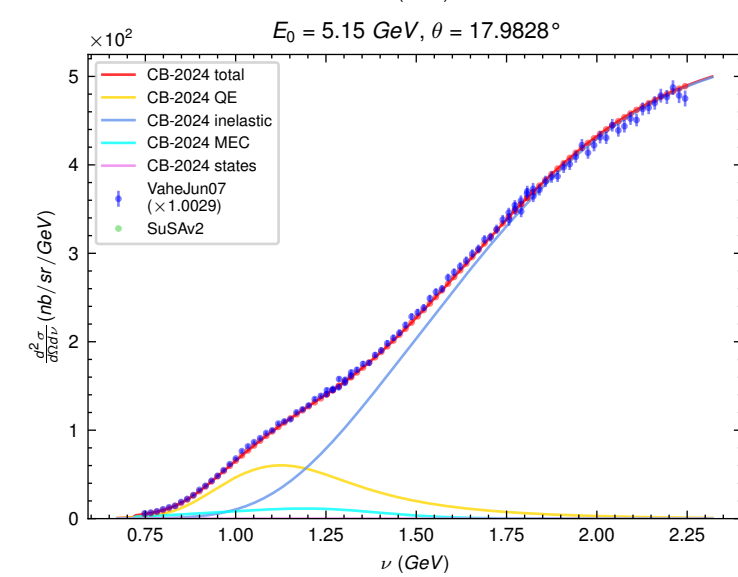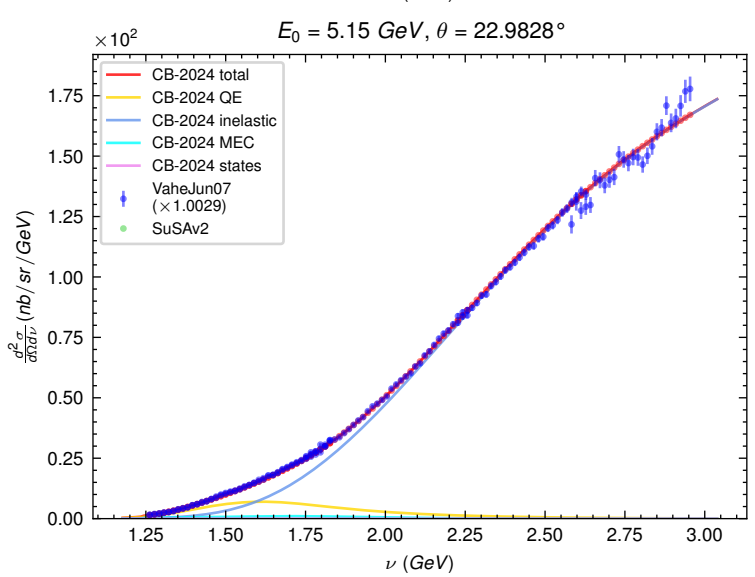



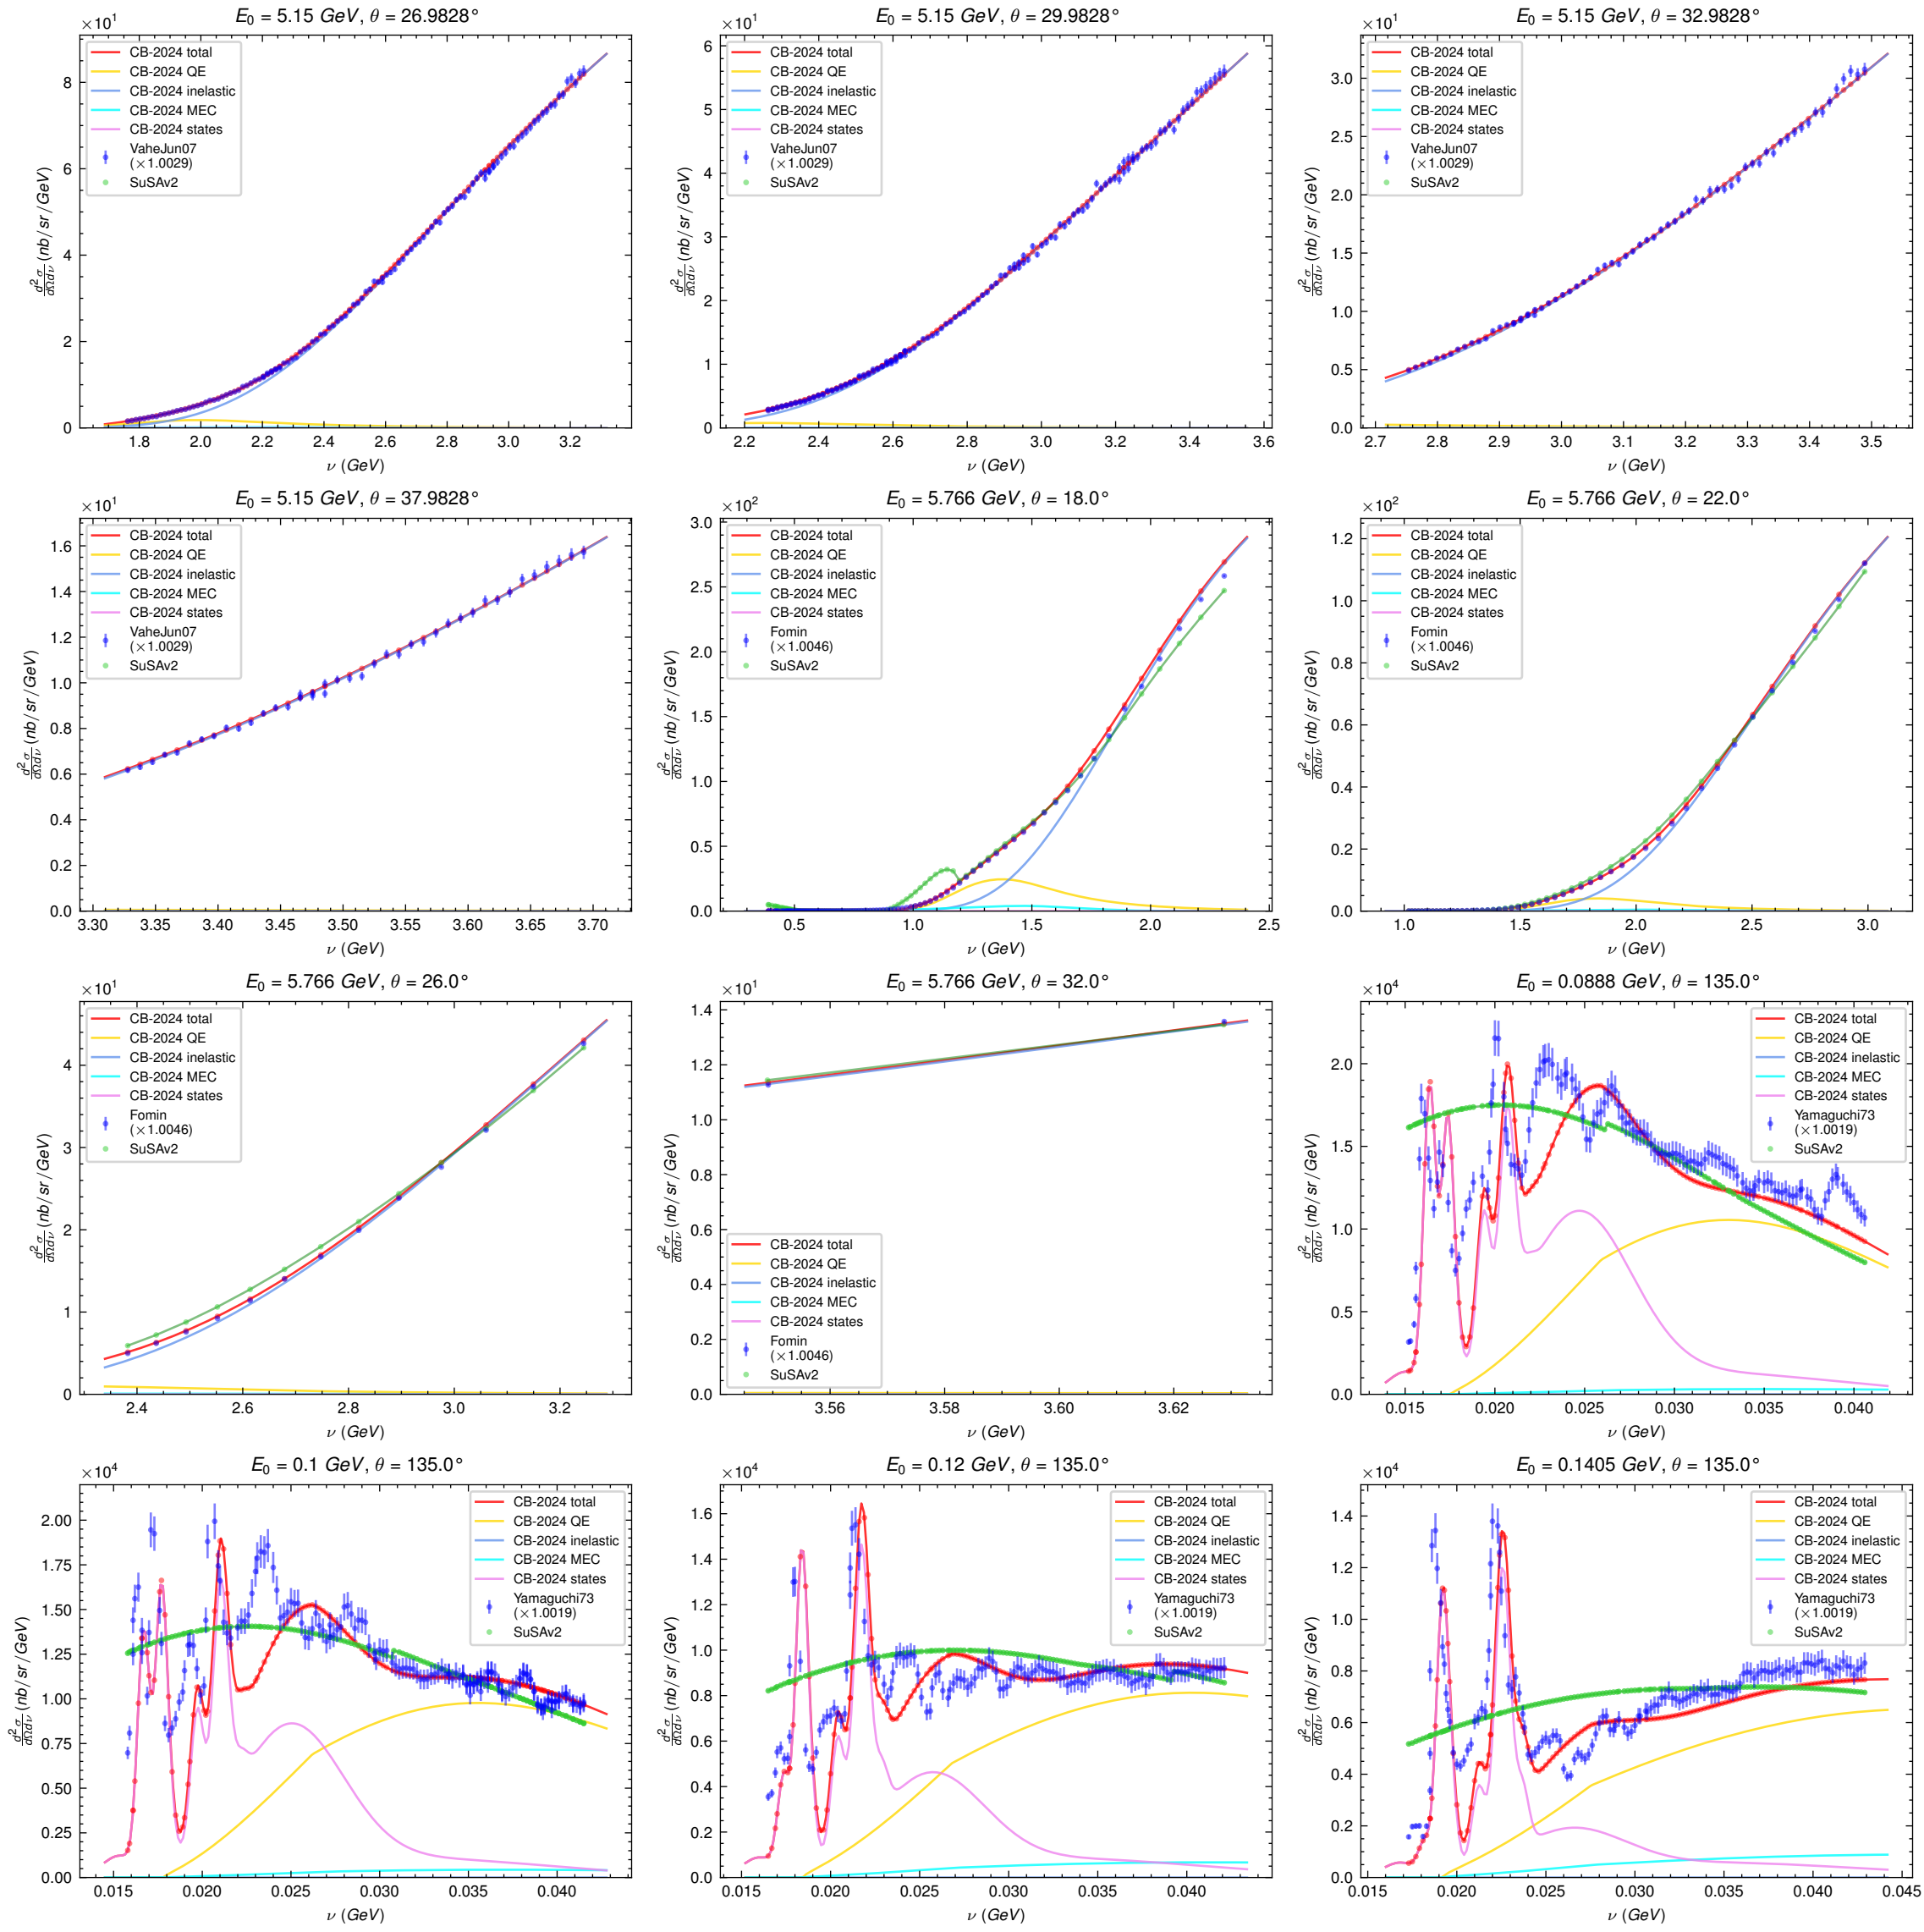

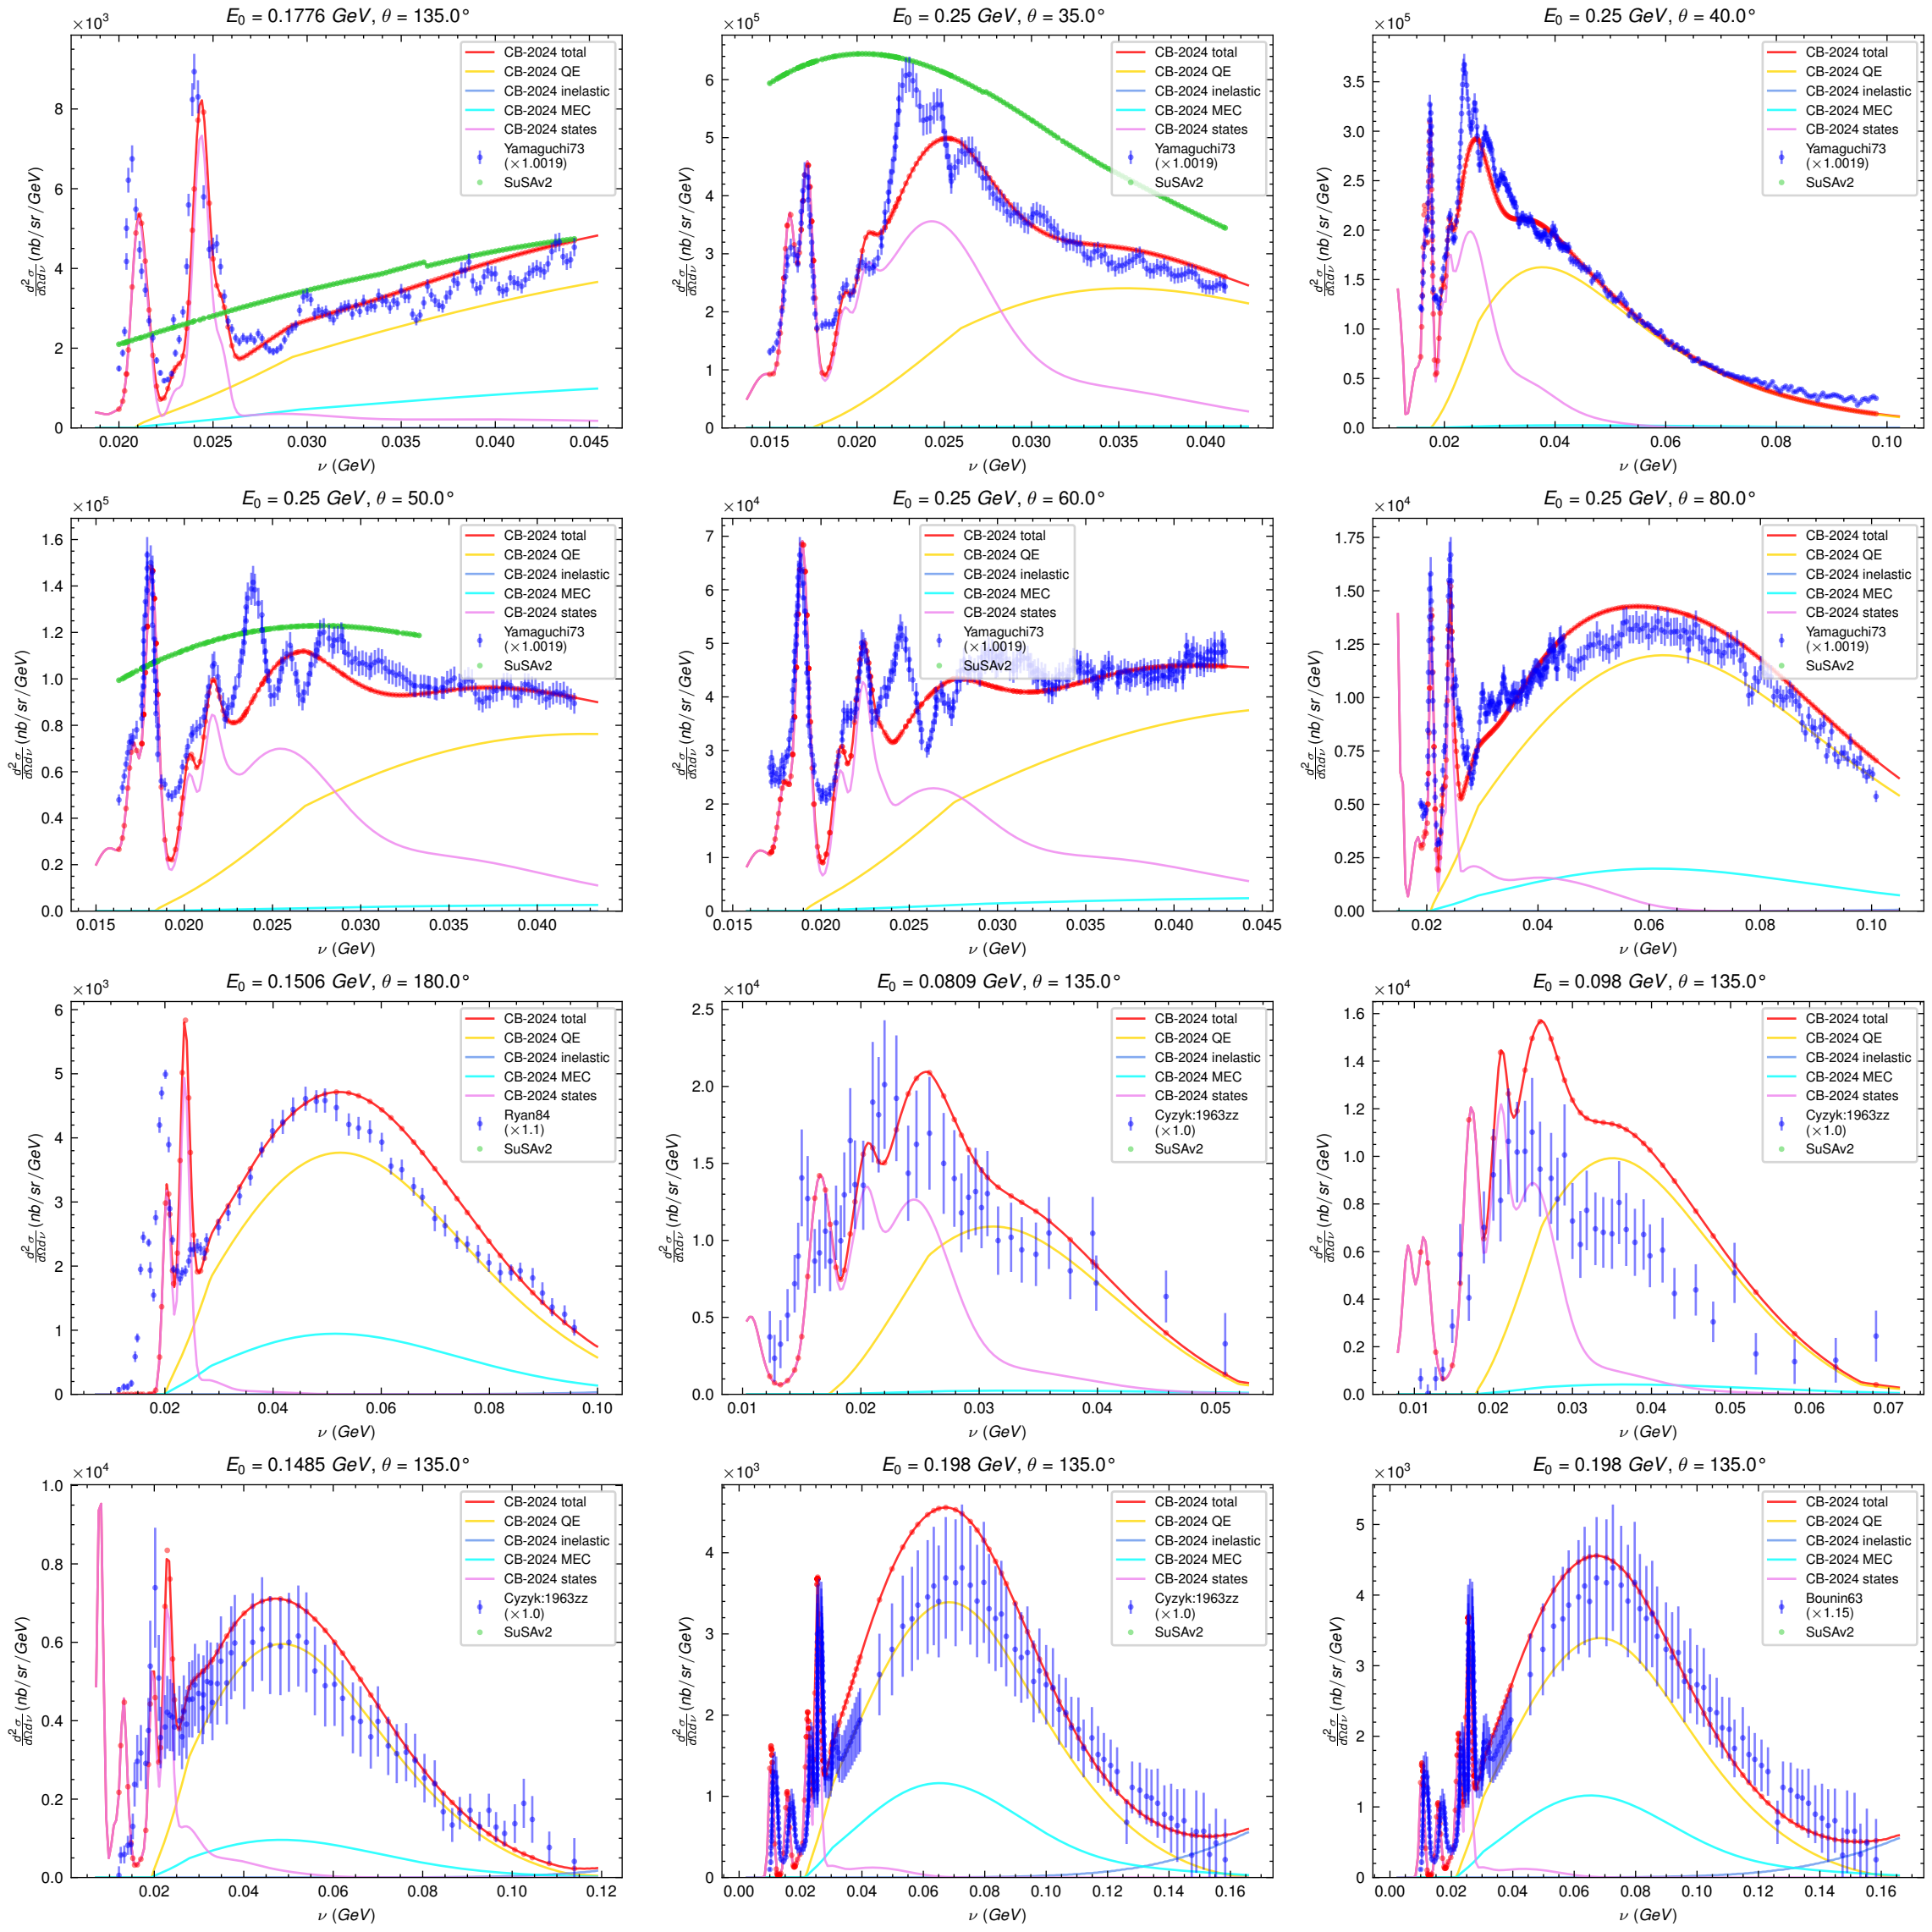

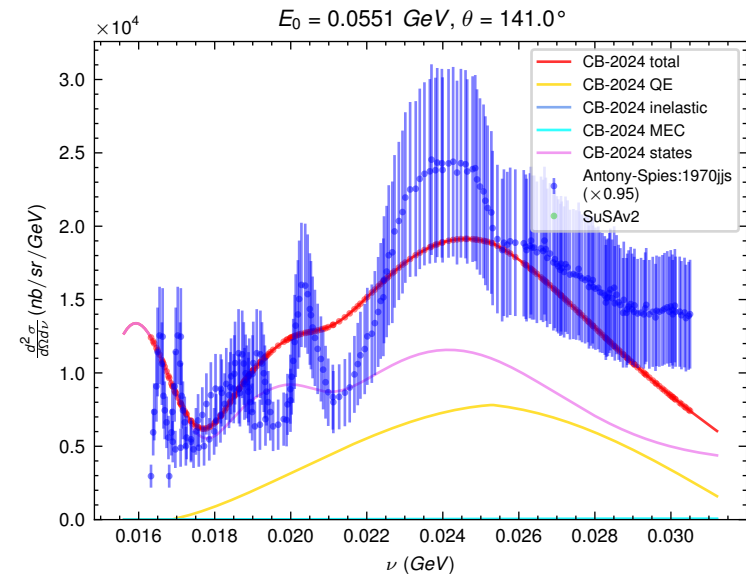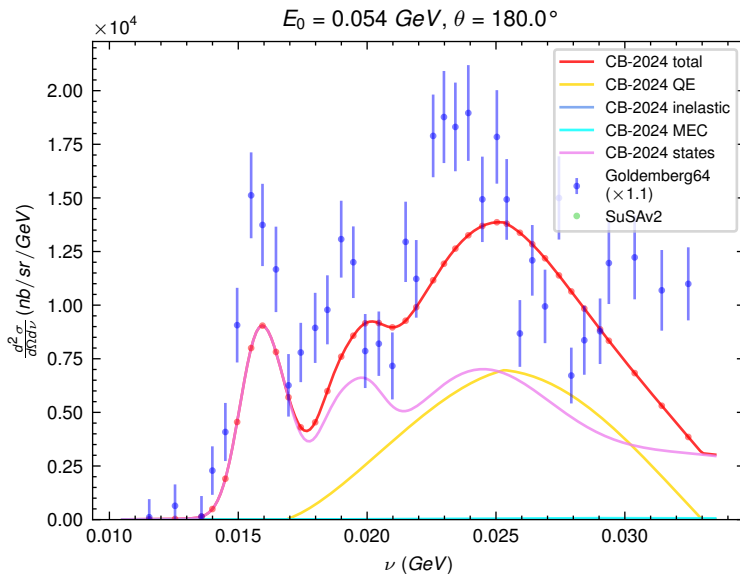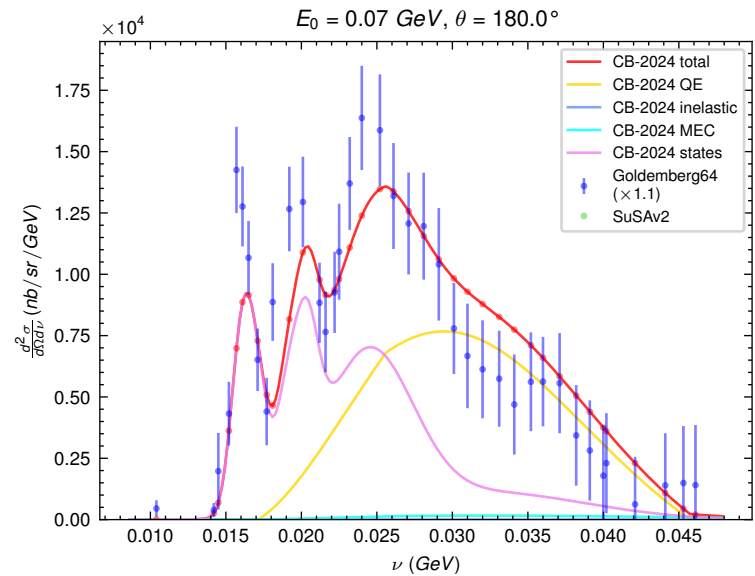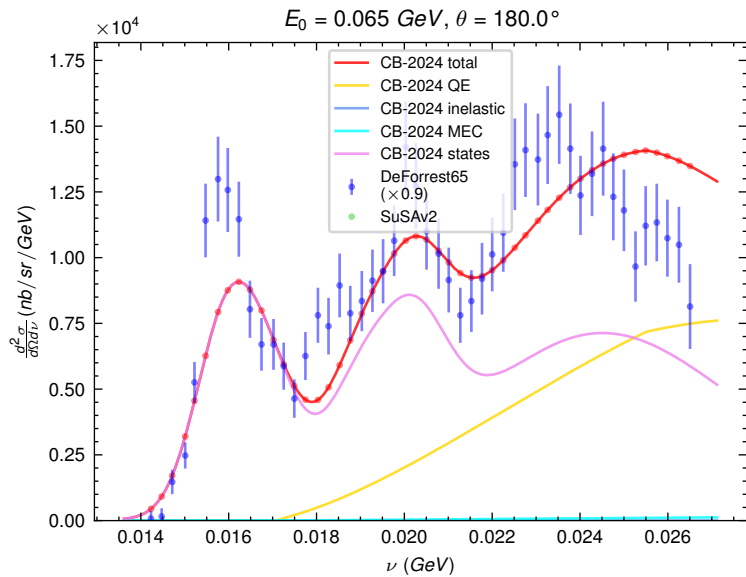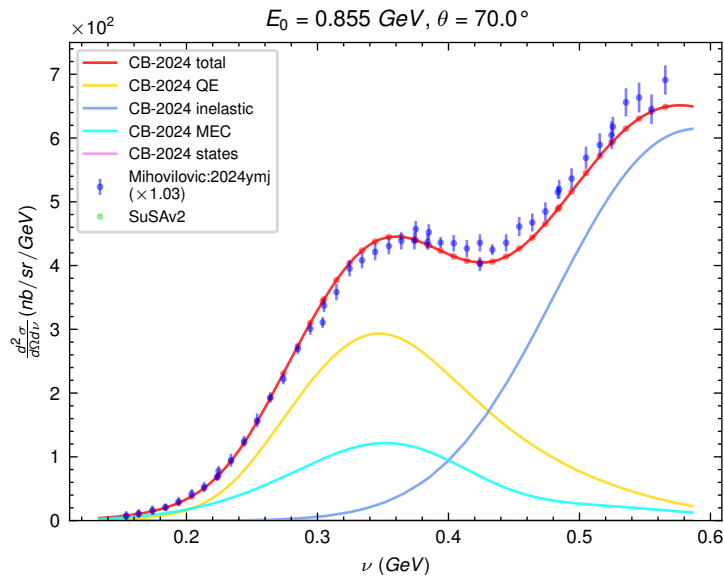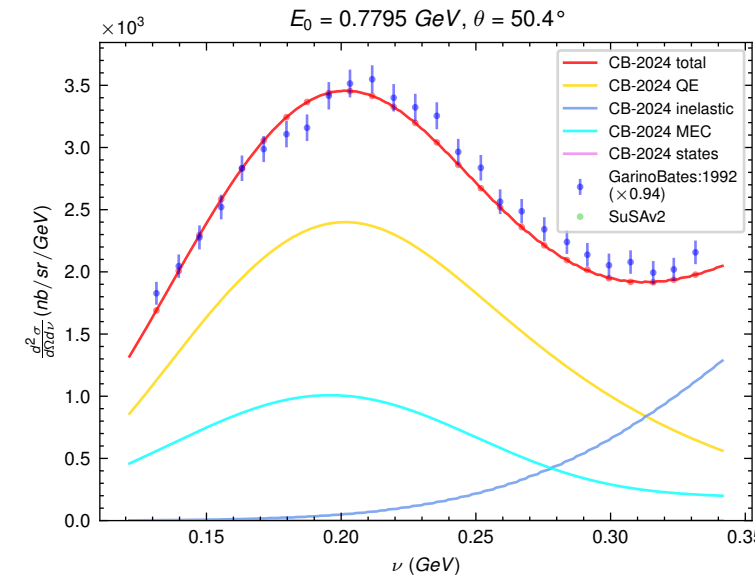

Supplement: Supplementary file 1 [file supp_cross.pdf]
